# Supplementary material for: Locally Differentially Private Minimum Finding
Source: arXiv:1905.11067 ancillary file (2019-05-27)
Supplement: Supplementary file 1 [file expr.pdf]

# Additional Experimental Results: Locally Differentially Private Minimum Finding

May 24, 2019

## 1 More Experiments: Synthetic Dataset

Here, we present the full experimental results on the synthetic datasets.

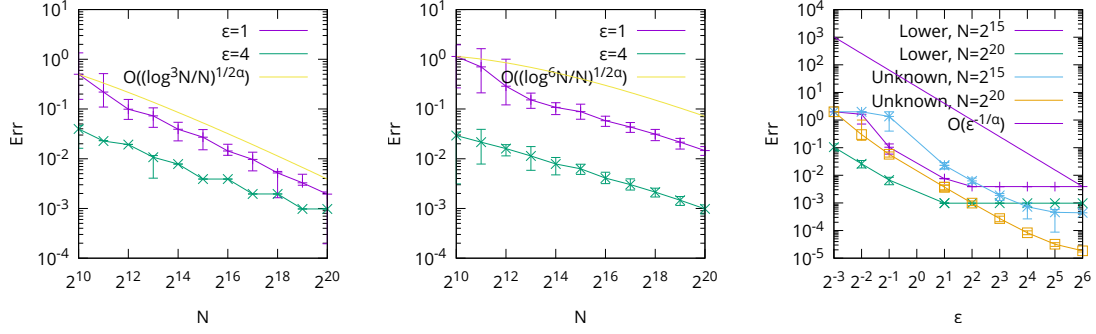

Figure 1: ( $\alpha = 0.5, \beta = 1, \Delta = 0.3$ , fixed) Err v.s.  $N$  (left and middle) and Err v.s.  $\epsilon$  (right). The left figure depicts the result with **Lower**  $\alpha$ , and the middle figure depicts the result with **Unknown**  $\alpha$ .

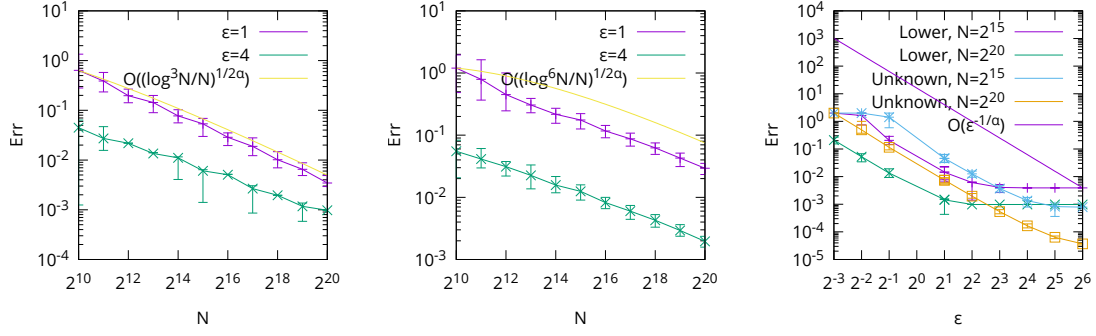

Figure 2: ( $\alpha = 0.5, \beta = 1, \Delta = 0.6$ , fixed) Err v.s.  $N$  (left and middle) and Err v.s.  $\epsilon$  (right). The left figure depicts the result with **Lower**  $\alpha$ , and the middle figure depicts the result with **Unknown**  $\alpha$ .

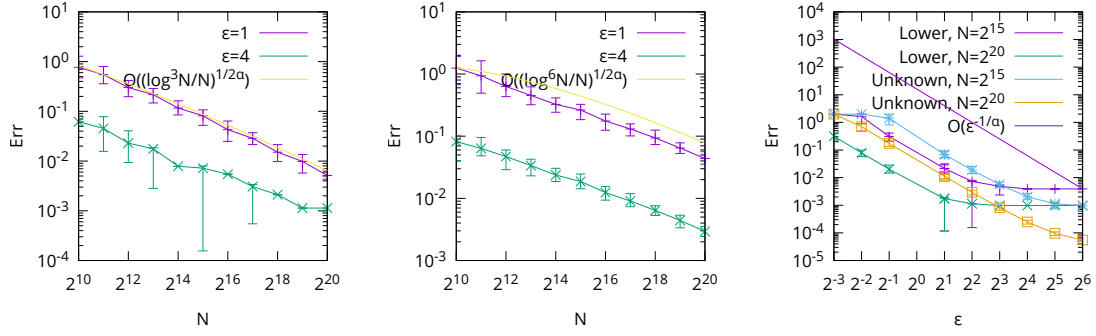

Figure 3: ( $\alpha = 0.5, \beta = 1, \Delta = 0.9$ , fixed) Err v.s.  $N$  (left and middle) and Err v.s.  $\epsilon$  (right). The left figure depicts the result with **Lower**  $\alpha$ , and the middle figure depicts the result with **Unknown**  $\alpha$ .

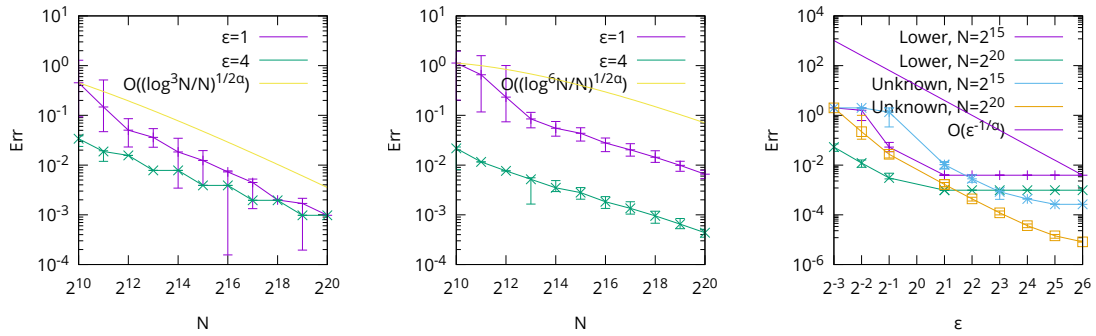

Figure 4: ( $\alpha = 0.5, \beta = 2, \Delta = 0.3$ , fixed) Err v.s.  $N$  (left and middle) and Err v.s.  $\epsilon$  (right). The left figure depicts the result with **Lower**  $\alpha$ , and the middle figure depicts the result with **Unknown**  $\alpha$ .

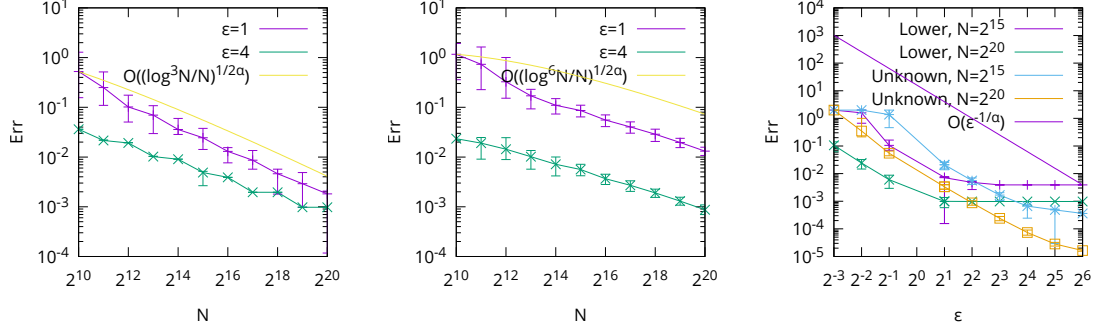

Figure 5: ( $\alpha = 0.5, \beta = 2, \Delta = 0.6$ , fixed) Err v.s.  $N$  (left and middle) and Err v.s.  $\epsilon$  (right). The left figure depicts the result with **Lower**  $\alpha$ , and the middle figure depicts the result with **Unknown**  $\alpha$ .

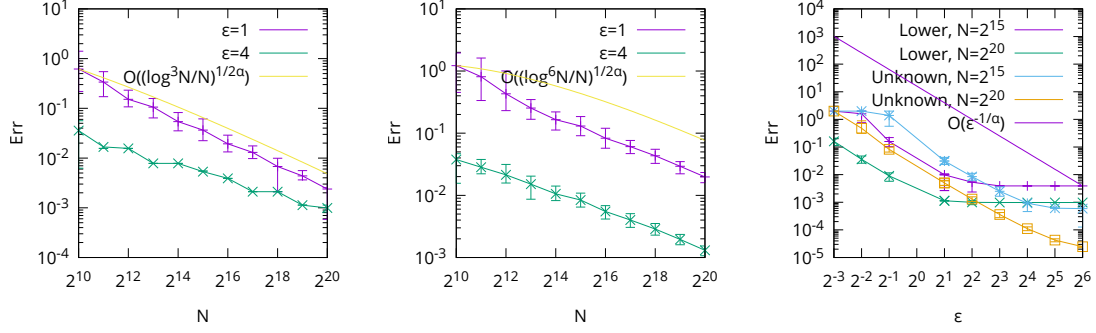

Figure 6: ( $\alpha = 0.5, \beta = 2, \Delta = 0.9$ , fixed) Err v.s.  $N$  (left and middle) and Err v.s.  $\epsilon$  (right). The left figure depicts the result with **Lower**  $\alpha$ , and the middle figure depicts the result with **Unknown**  $\alpha$ .

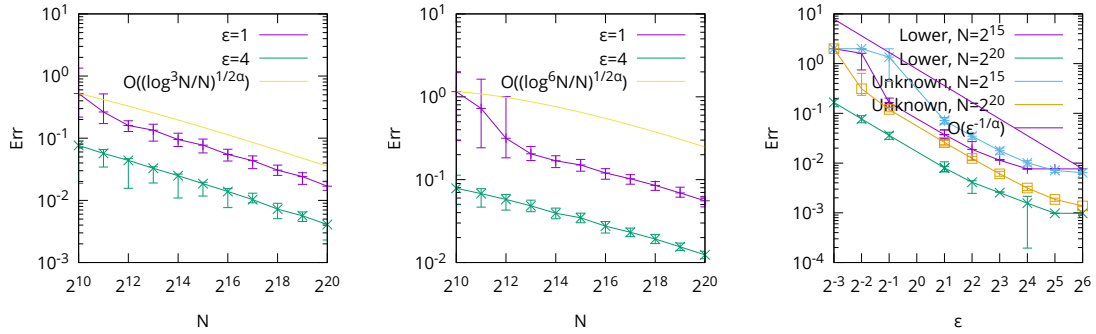

Figure 7: ( $\alpha = 0.9, \beta = 1, \Delta = 0.3$ , fixed) Err v.s.  $N$  (left and middle) and Err v.s.  $\epsilon$  (right). The left figure depicts the result with **Lower**  $\alpha$ , and the middle figure depicts the result with **Unknown**  $\alpha$ .

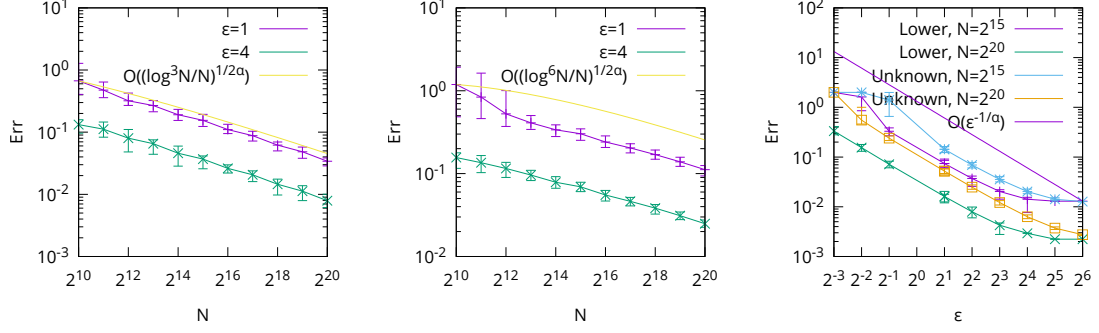

Figure 8: ( $\alpha = 0.9, \beta = 1, \Delta = 0.6$ , fixed) Err v.s.  $N$  (left and middle) and Err v.s.  $\epsilon$  (right). The left figure depicts the result with **Lower**  $\alpha$ , and the middle figure depicts the result with **Unknown**  $\alpha$ .

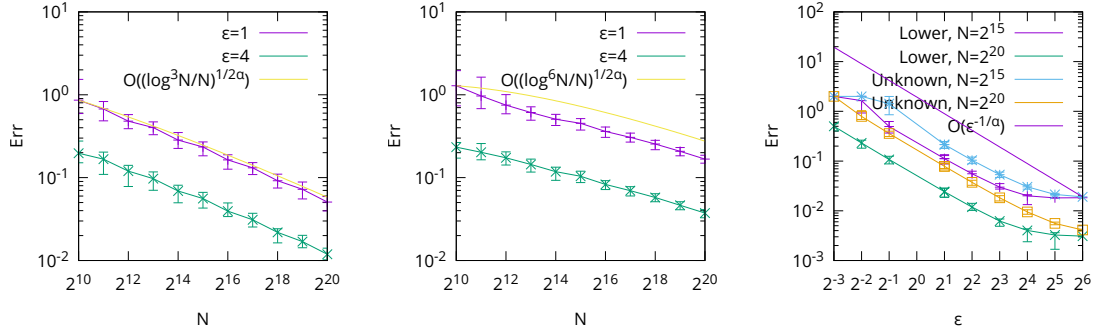

Figure 9: ( $\alpha = 0.9, \beta = 1, \Delta = 0.9$ , fixed) Err v.s.  $N$  (left and middle) and Err v.s.  $\epsilon$  (right). The left figure depicts the result with **Lower**  $\alpha$ , and the middle figure depicts the result with **Unknown**  $\alpha$ .

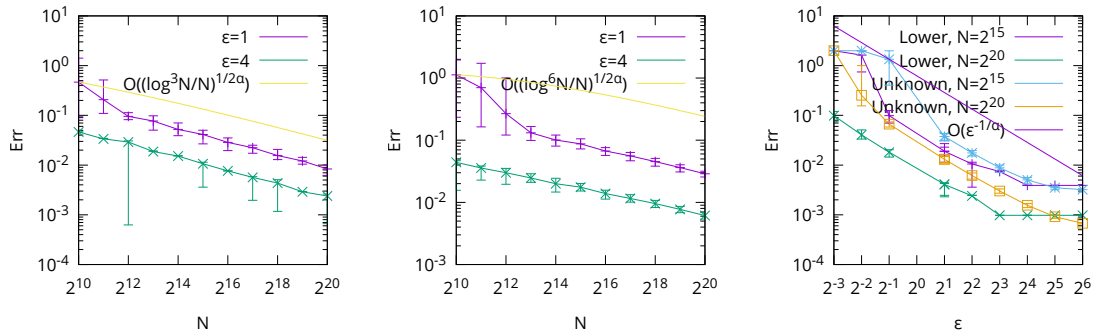

Figure 10: ( $\alpha = 0.9, \beta = 2, \Delta = 0.3$ , fixed) Err v.s.  $N$  (left and middle) and Err v.s.  $\epsilon$  (right). The left figure depicts the result with **Lower**  $\alpha$ , and the middle figure depicts the result with **Unknown**  $\alpha$ .

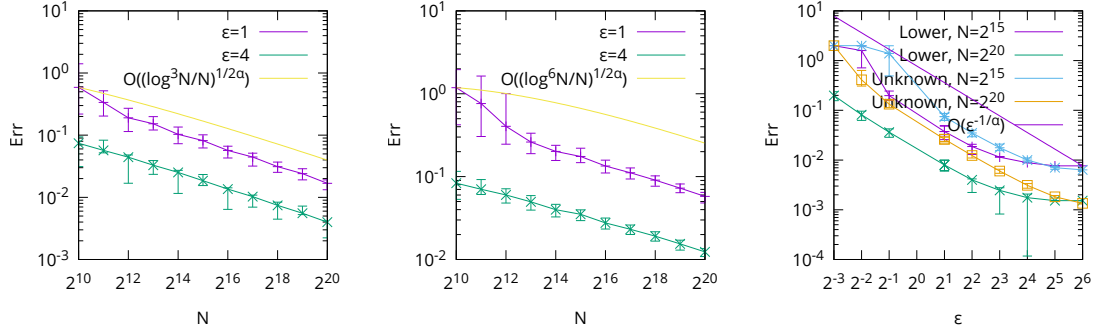

Figure 11: ( $\alpha = 0.9$ ,  $\beta = 2$ ,  $\Delta = 0.6$ , fixed) Err v.s.  $N$  (left and middle) and Err v.s.  $\epsilon$  (right). The left figure depicts the result with **Lower**  $\alpha$ , and the middle figure depicts the result with **Unknown**  $\alpha$ .

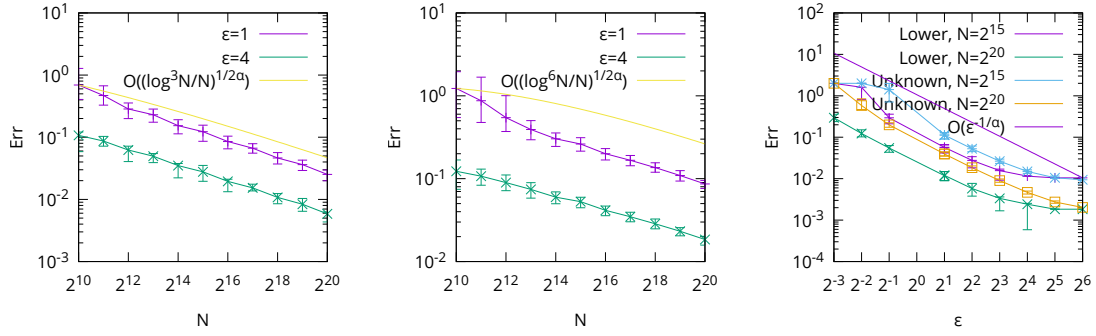

Figure 12: ( $\alpha = 0.9$ ,  $\beta = 2$ ,  $\Delta = 0.9$ , fixed) Err v.s.  $N$  (left and middle) and Err v.s.  $\epsilon$  (right). The left figure depicts the result with **Lower**  $\alpha$ , and the middle figure depicts the result with **Unknown**  $\alpha$ .

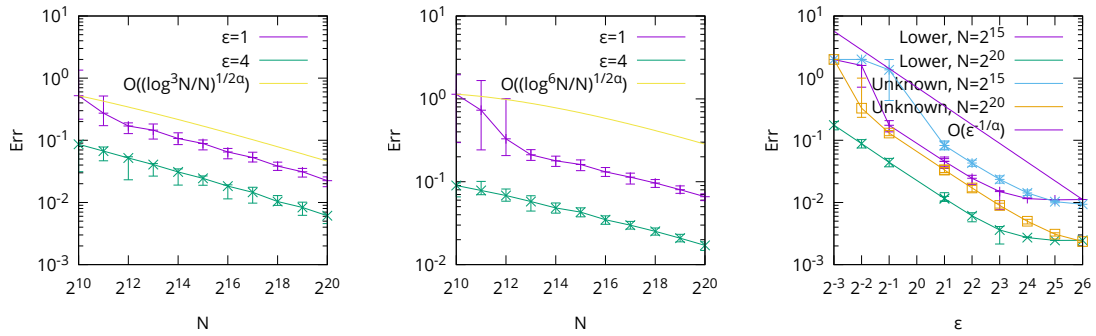

Figure 13: ( $\alpha = 1$ ,  $\beta = 1$ ,  $\Delta = 0.3$ , fixed) Err v.s.  $N$  (left and middle) and Err v.s.  $\epsilon$  (right). The left figure depicts the result with **Lower**  $\alpha$ , and the middle figure depicts the result with **Unknown**  $\alpha$ .

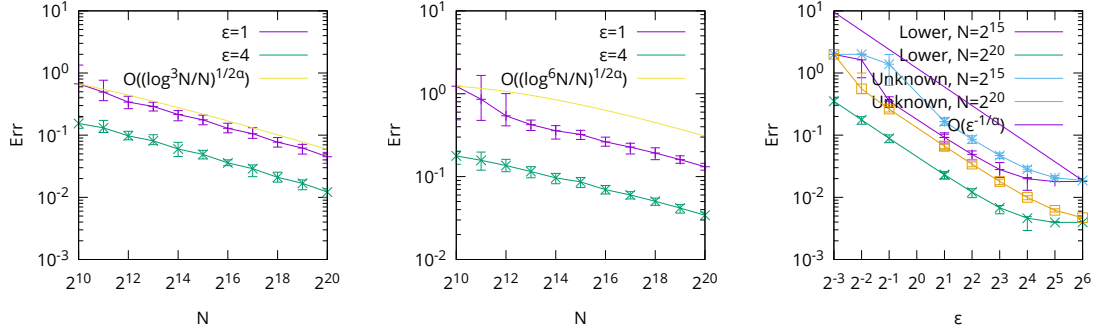

Figure 14: ( $\alpha = 1, \beta = 1, \Delta = 0.6$ , fixed) Err v.s.  $N$  (left and middle) and Err v.s.  $\epsilon$  (right). The left figure depicts the result with **Lower**  $\alpha$ , and the middle figure depicts the result with **Unknown**  $\alpha$ .

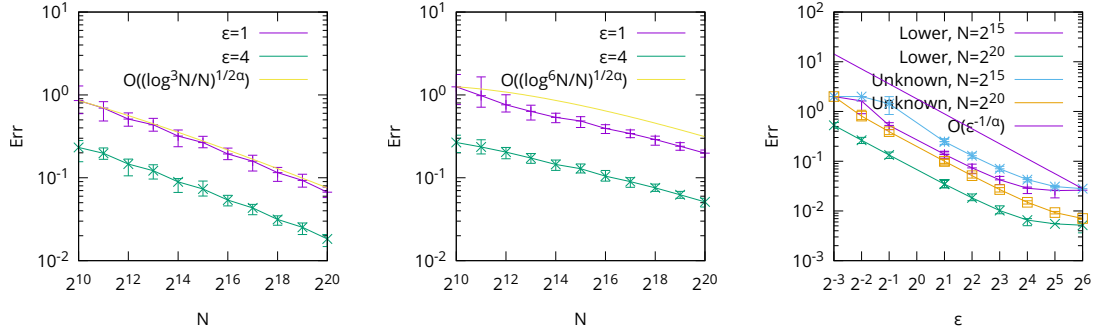

Figure 15: ( $\alpha = 1, \beta = 1, \Delta = 0.9$ , fixed) Err v.s.  $N$  (left and middle) and Err v.s.  $\epsilon$  (right). The left figure depicts the result with **Lower**  $\alpha$ , and the middle figure depicts the result with **Unknown**  $\alpha$ .

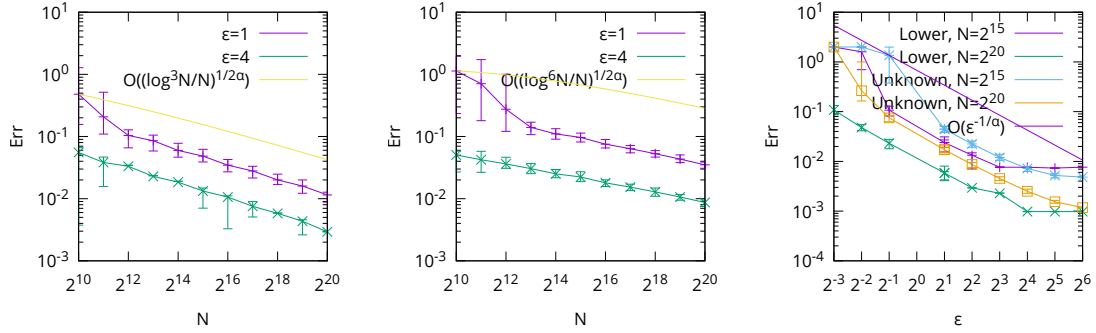

Figure 16: ( $\alpha = 1, \beta = 2, \Delta = 0.3$ , fixed) Err v.s.  $N$  (left and middle) and Err v.s.  $\epsilon$  (right). The left figure depicts the result with **Lower**  $\alpha$ , and the middle figure depicts the result with **Unknown**  $\alpha$ .

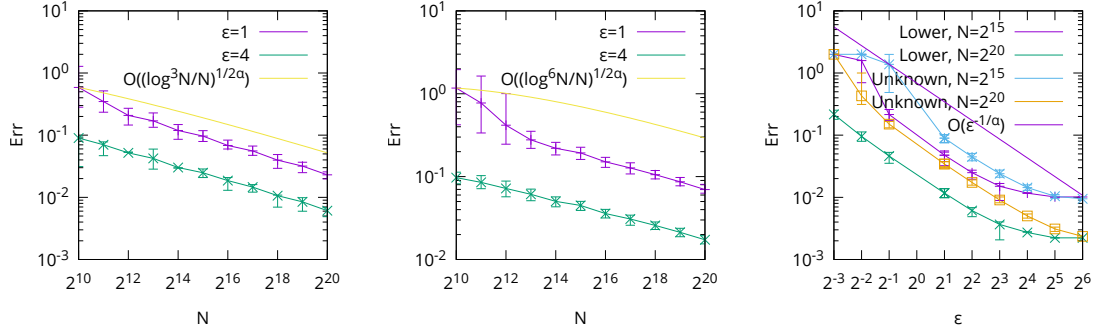

Figure 17: ( $\alpha = 1, \beta = 2, \Delta = 0.6$ , fixed) Err v.s.  $N$  (left and middle) and Err v.s.  $\epsilon$  (right). The left figure depicts the result with **Lower**  $\alpha$ , and the middle figure depicts the result with **Unknown**  $\alpha$ .

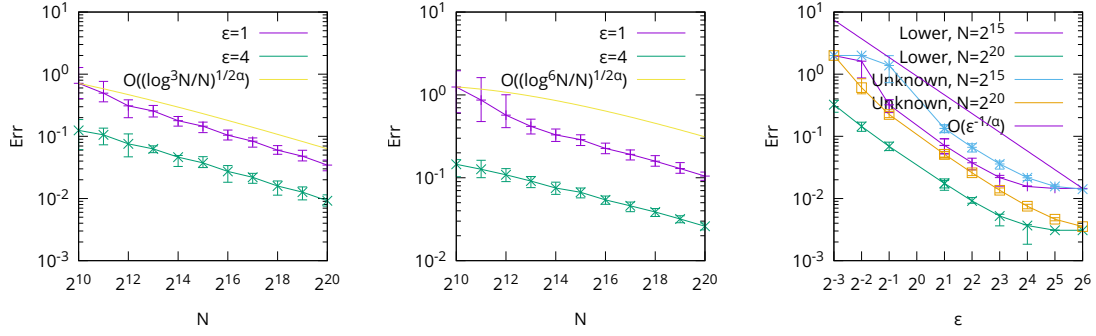

Figure 18: ( $\alpha = 1, \beta = 2, \Delta = 0.9$ , fixed) Err v.s.  $N$  (left and middle) and Err v.s.  $\epsilon$  (right). The left figure depicts the result with **Lower**  $\alpha$ , and the middle figure depicts the result with **Unknown**  $\alpha$ .

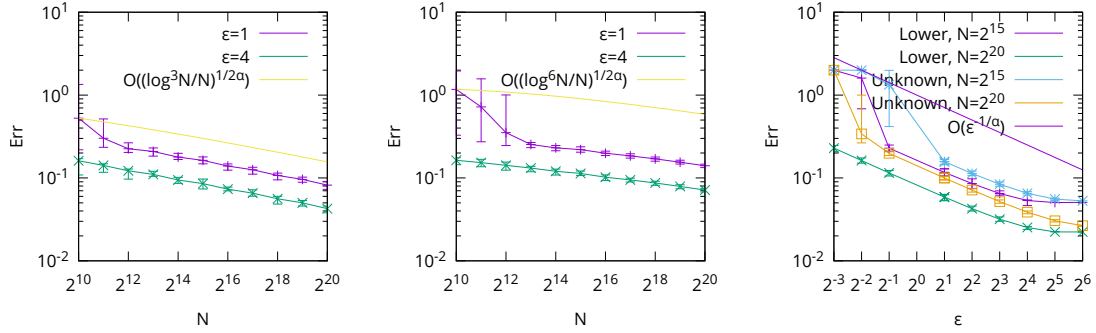

Figure 19: ( $\alpha = 2, \beta = 1, \Delta = 0.3$ , fixed) Err v.s.  $N$  (left and middle) and Err v.s.  $\epsilon$  (right). The left figure depicts the result with **Lower**  $\alpha$ , and the middle figure depicts the result with **Unknown**  $\alpha$ .

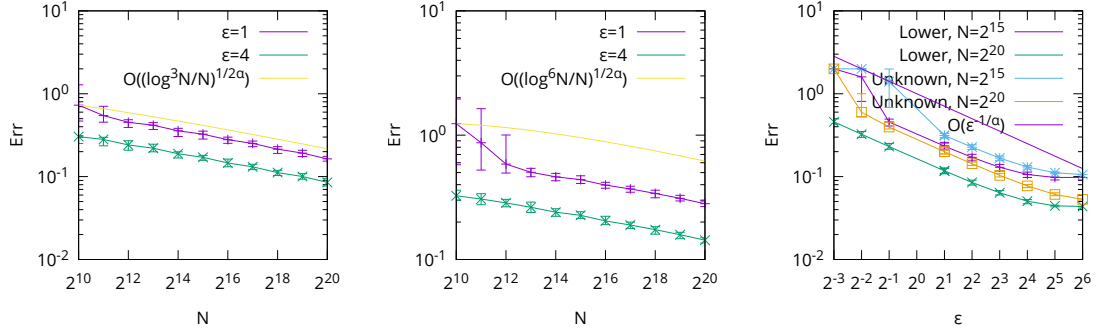

Figure 20: ( $\alpha = 2, \beta = 1, \Delta = 0.6$ , fixed) Err v.s.  $N$  (left and middle) and Err v.s.  $\epsilon$  (right). The left figure depicts the result with **Lower**  $\alpha$ , and the middle figure depicts the result with **Unknown**  $\alpha$ .

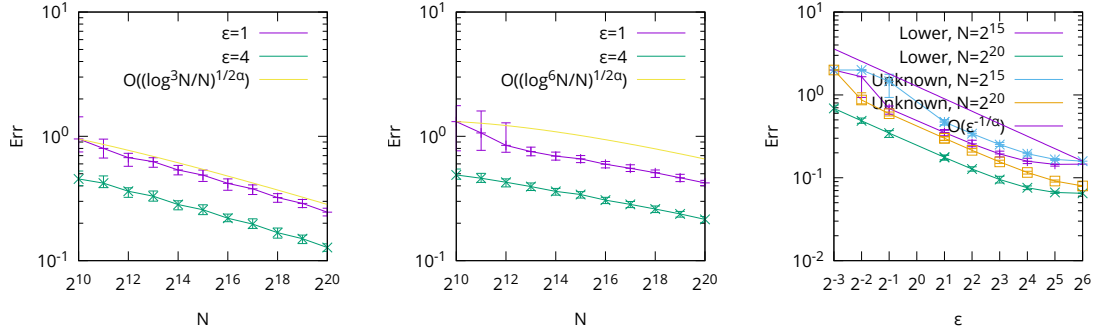

Figure 21: ( $\alpha = 2, \beta = 1, \Delta = 0.9$ , fixed) Err v.s.  $N$  (left and middle) and Err v.s.  $\epsilon$  (right). The left figure depicts the result with **Lower**  $\alpha$ , and the middle figure depicts the result with **Unknown**  $\alpha$ .

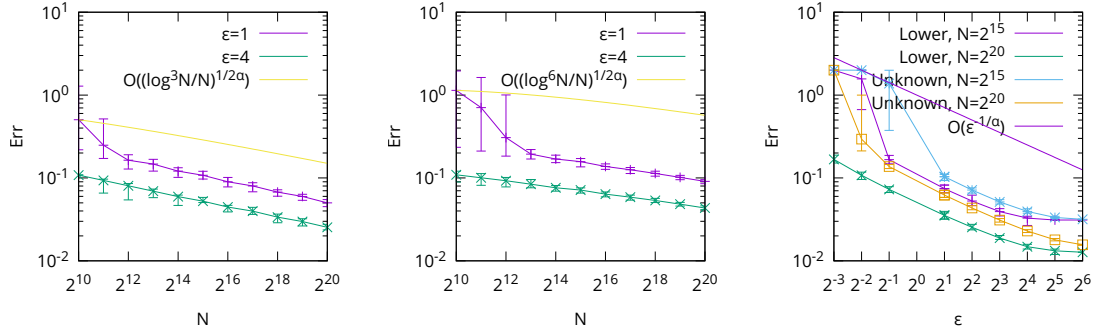

Figure 22: ( $\alpha = 2, \beta = 2, \Delta = 0.3$ , fixed) Err v.s.  $N$  (left and middle) and Err v.s.  $\epsilon$  (right). The left figure depicts the result with **Lower**  $\alpha$ , and the middle figure depicts the result with **Unknown**  $\alpha$ .



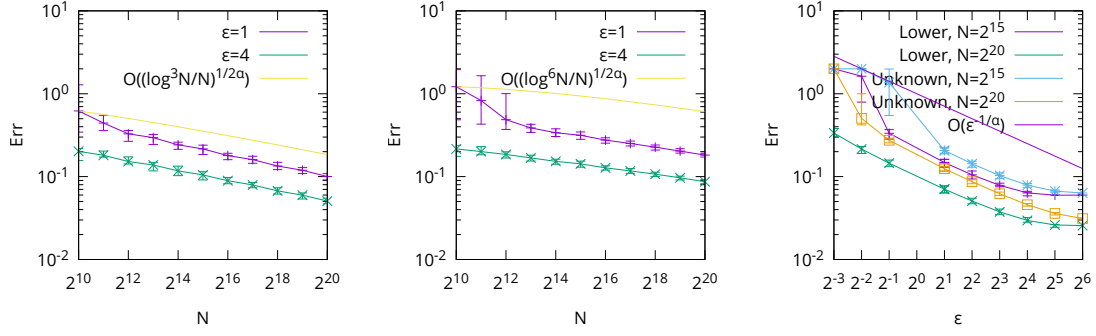

Figure 23: ( $\alpha = 2, \beta = 2, \Delta = 0.6$ , fixed) Err v.s.  $N$  (left and middle) and Err v.s.  $\epsilon$  (right). The left figure depicts the result with **Lower**  $\alpha$ , and the middle figure depicts the result with **Unknown**  $\alpha$ .

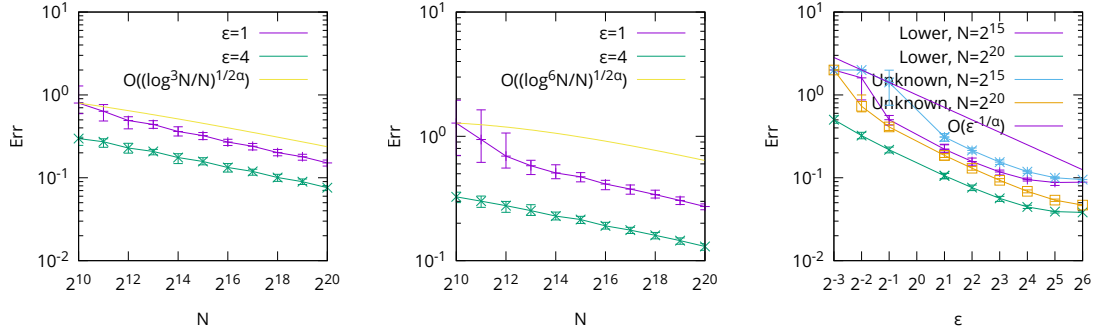

Figure 24: ( $\alpha = 2, \beta = 2, \Delta = 0.9$ , fixed) Err v.s.  $N$  (left and middle) and Err v.s.  $\epsilon$  (right). The left figure depicts the result with **Lower**  $\alpha$ , and the middle figure depicts the result with **Unknown**  $\alpha$ .

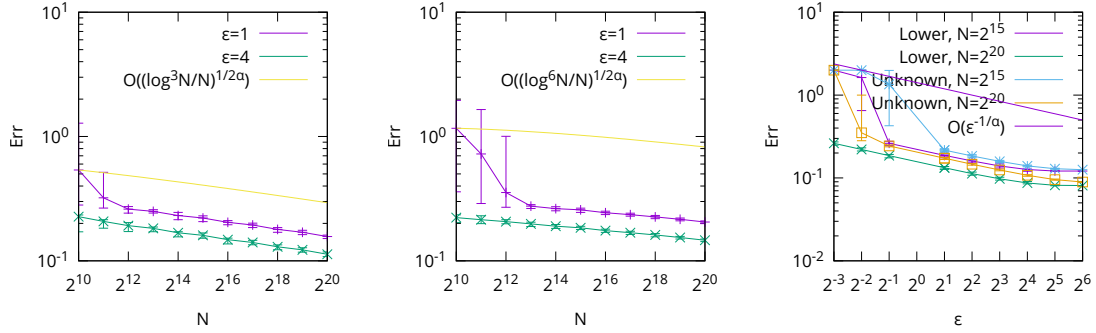

Figure 25: ( $\alpha = 4, \beta = 1, \Delta = 0.3$ , fixed) Err v.s.  $N$  (left and middle) and Err v.s.  $\epsilon$  (right). The left figure depicts the result with **Lower**  $\alpha$ , and the middle figure depicts the result with **Unknown**  $\alpha$ .

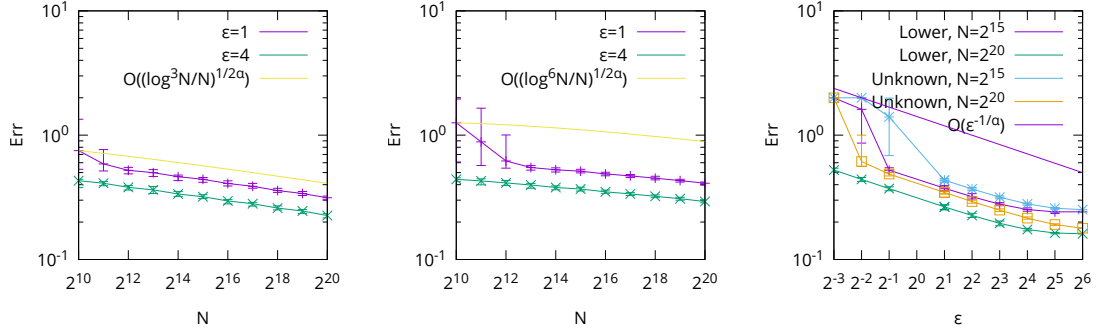

Figure 26: ( $\alpha = 4, \beta = 1, \Delta = 0.6$ , fixed) Err v.s.  $N$  (left and middle) and Err v.s.  $\epsilon$  (right). The left figure depicts the result with **Lower**  $\alpha$ , and the middle figure depicts the result with **Unknown**  $\alpha$ .

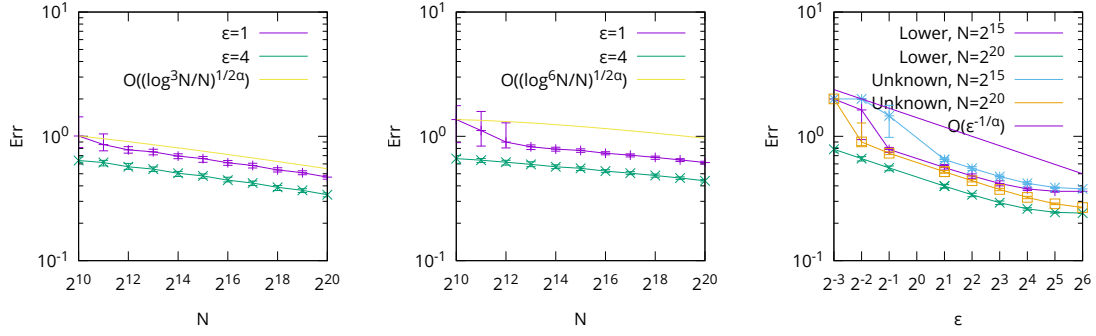

Figure 27: ( $\alpha = 4, \beta = 1, \Delta = 0.9$ , fixed) Err v.s.  $N$  (left and middle) and Err v.s.  $\epsilon$  (right). The left figure depicts the result with **Lower**  $\alpha$ , and the middle figure depicts the result with **Unknown**  $\alpha$ .

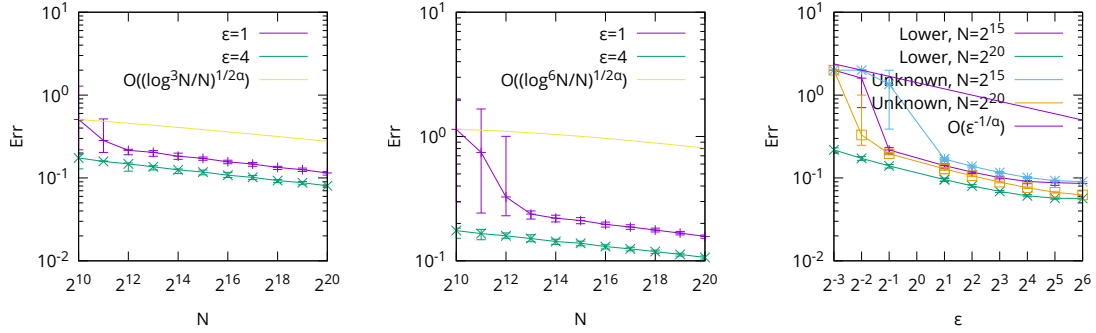

Figure 28: ( $\alpha = 4, \beta = 2, \Delta = 0.3$ , fixed) Err v.s.  $N$  (left and middle) and Err v.s.  $\epsilon$  (right). The left figure depicts the result with **Lower**  $\alpha$ , and the middle figure depicts the result with **Unknown**  $\alpha$ .

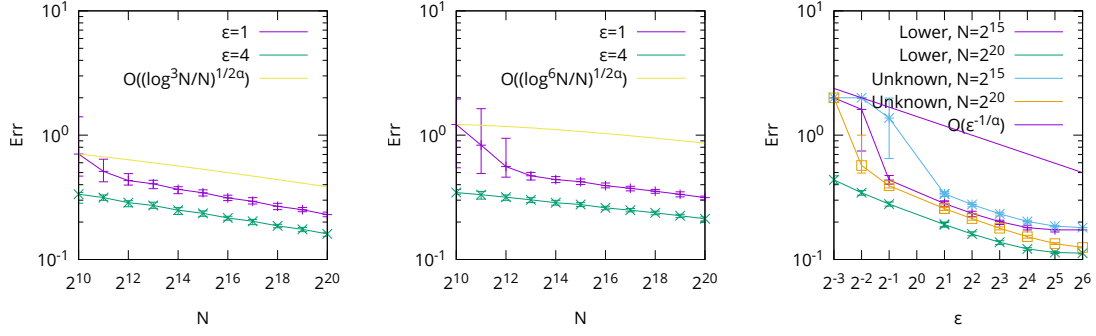

Figure 29: ( $\alpha = 4, \beta = 2, \Delta = 0.6$ , fixed) Err v.s.  $N$  (left and middle) and Err v.s.  $\epsilon$  (right). The left figure depicts the result with **Lower**  $\alpha$ , and the middle figure depicts the result with **Unknown**  $\alpha$ .

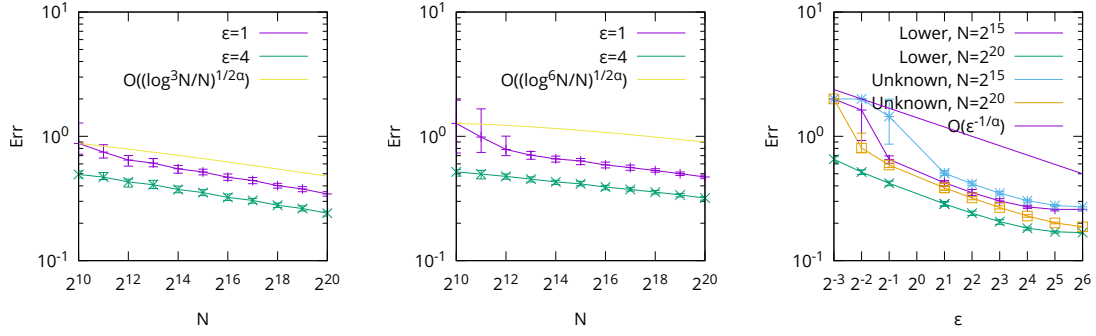

Figure 30: ( $\alpha = 4, \beta = 2, \Delta = 0.9$ , fixed) Err v.s.  $N$  (left and middle) and Err v.s.  $\epsilon$  (right). The left figure depicts the result with **Lower**  $\alpha$ , and the middle figure depicts the result with **Unknown**  $\alpha$ .

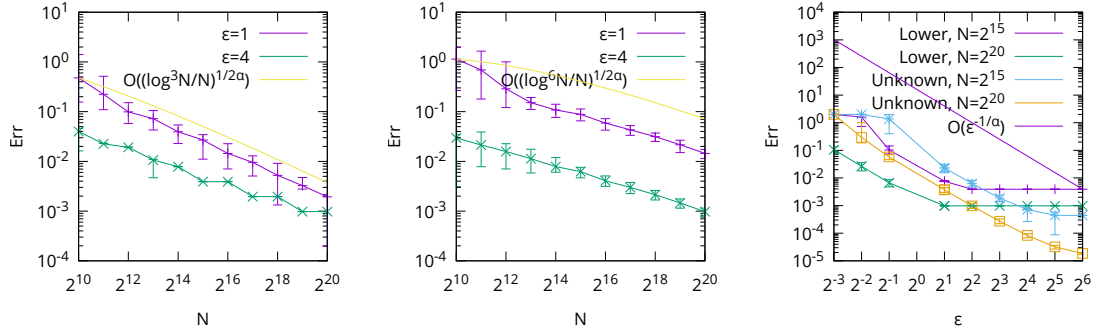

Figure 31: ( $\alpha = 0.5, \beta = 1, \Delta = 0.3$ , iid) Err v.s.  $N$  (left and middle) and Err v.s.  $\epsilon$  (right). The left figure depicts the result with **Lower**  $\alpha$ , and the middle figure depicts the result with **Unknown**  $\alpha$ .

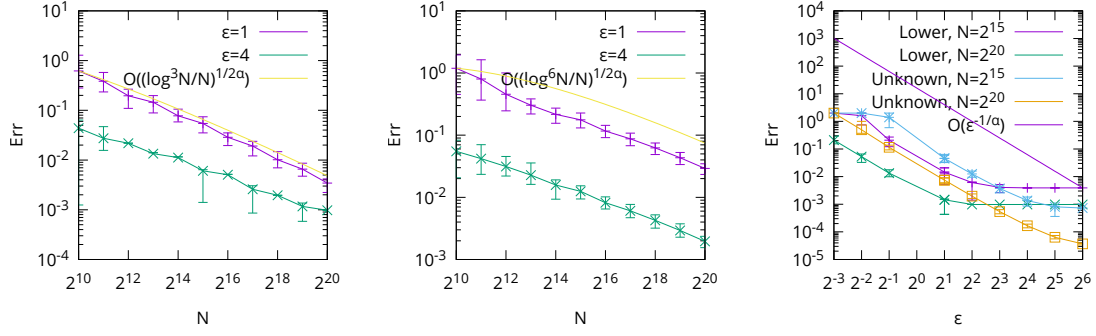

Figure 32: ( $\alpha = 0.5$ ,  $\beta = 1$ ,  $\Delta = 0.6$ , iid) Err v.s.  $N$  (left and middle) and Err v.s.  $\epsilon$  (right). The left figure depicts the result with **Lower**  $\alpha$ , and the middle figure depicts the result with **Unknown**  $\alpha$ .

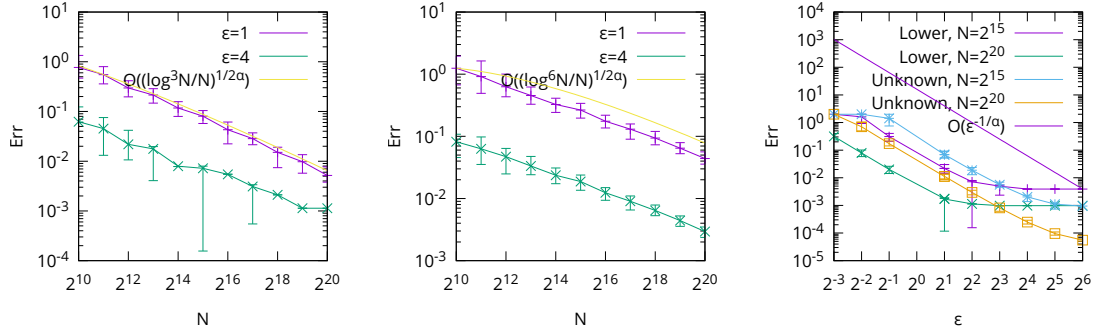

Figure 33: ( $\alpha = 0.5$ ,  $\beta = 1$ ,  $\Delta = 0.9$ , iid) Err v.s.  $N$  (left and middle) and Err v.s.  $\epsilon$  (right). The left figure depicts the result with **Lower**  $\alpha$ , and the middle figure depicts the result with **Unknown**  $\alpha$ .

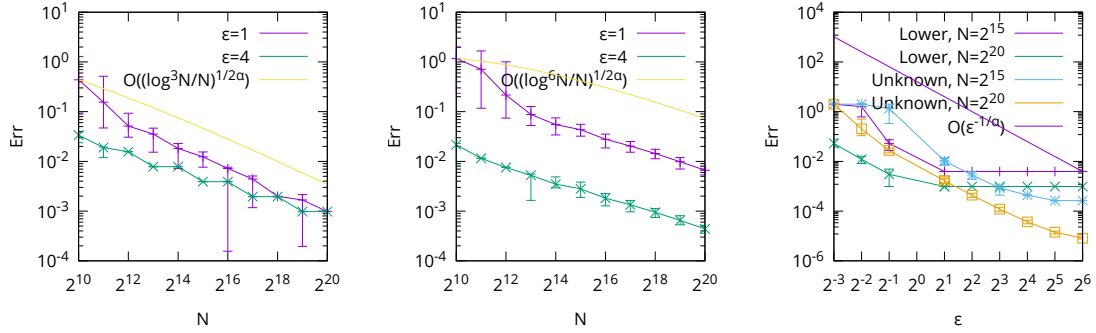

Figure 34: ( $\alpha = 0.5$ ,  $\beta = 2$ ,  $\Delta = 0.3$ , iid) Err v.s.  $N$  (left and middle) and Err v.s.  $\epsilon$  (right). The left figure depicts the result with **Lower**  $\alpha$ , and the middle figure depicts the result with **Unknown**  $\alpha$ .

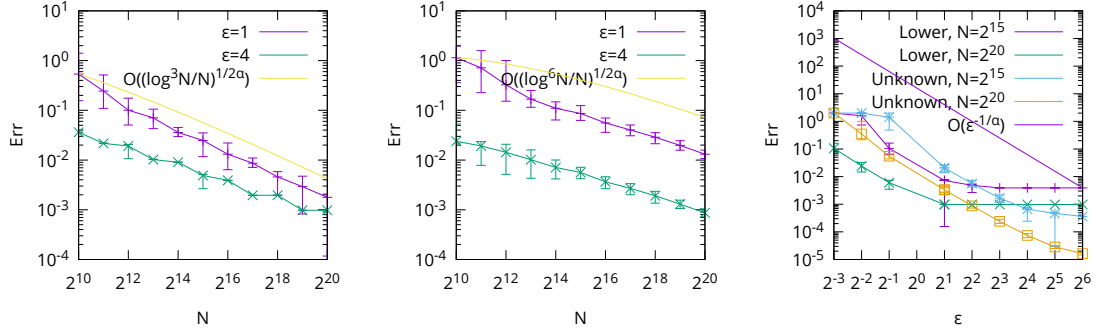

Figure 35: ( $\alpha = 0.5$ ,  $\beta = 2$ ,  $\Delta = 0.6$ , iid) Err v.s.  $N$  (left and middle) and Err v.s.  $\epsilon$  (right). The left figure depicts the result with **Lower**  $\alpha$ , and the middle figure depicts the result with **Unknown**  $\alpha$ .

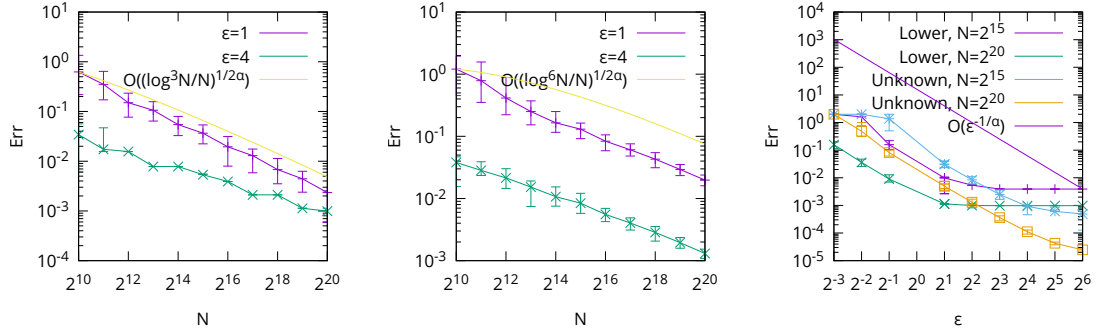

Figure 36: ( $\alpha = 0.5$ ,  $\beta = 2$ ,  $\Delta = 0.9$ , iid) Err v.s.  $N$  (left and middle) and Err v.s.  $\epsilon$  (right). The left figure depicts the result with **Lower**  $\alpha$ , and the middle figure depicts the result with **Unknown**  $\alpha$ .

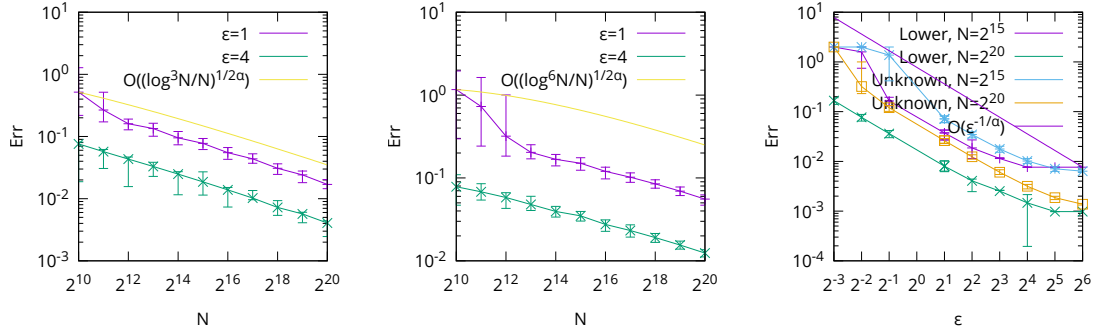

Figure 37: ( $\alpha = 0.9$ ,  $\beta = 1$ ,  $\Delta = 0.3$ , iid) Err v.s.  $N$  (left and middle) and Err v.s.  $\epsilon$  (right). The left figure depicts the result with **Lower**  $\alpha$ , and the middle figure depicts the result with **Unknown**  $\alpha$ .

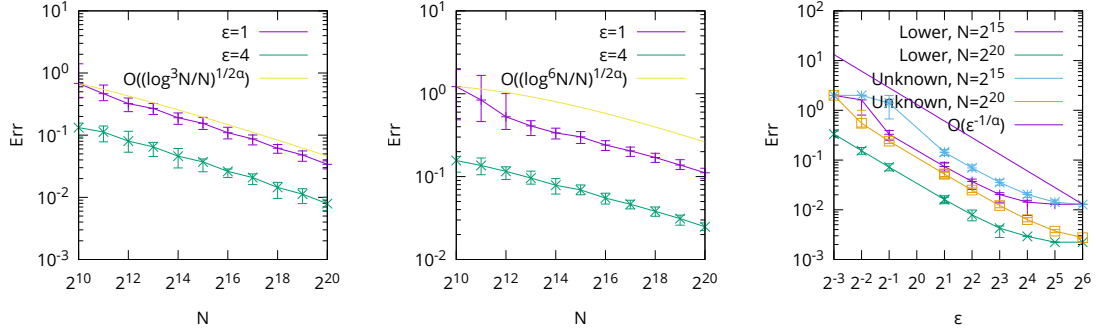

Figure 38: ( $\alpha = 0.9, \beta = 1, \Delta = 0.6$ , iid) Err v.s.  $N$  (left and middle) and Err v.s.  $\epsilon$  (right). The left figure depicts the result with **Lower**  $\alpha$ , and the middle figure depicts the result with **Unknown**  $\alpha$ .

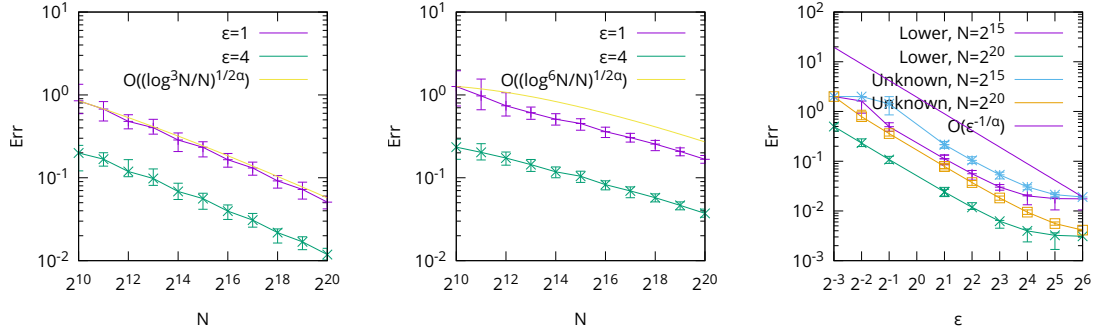

Figure 39: ( $\alpha = 0.9, \beta = 1, \Delta = 0.9$ , iid) Err v.s.  $N$  (left and middle) and Err v.s.  $\epsilon$  (right). The left figure depicts the result with **Lower**  $\alpha$ , and the middle figure depicts the result with **Unknown**  $\alpha$ .

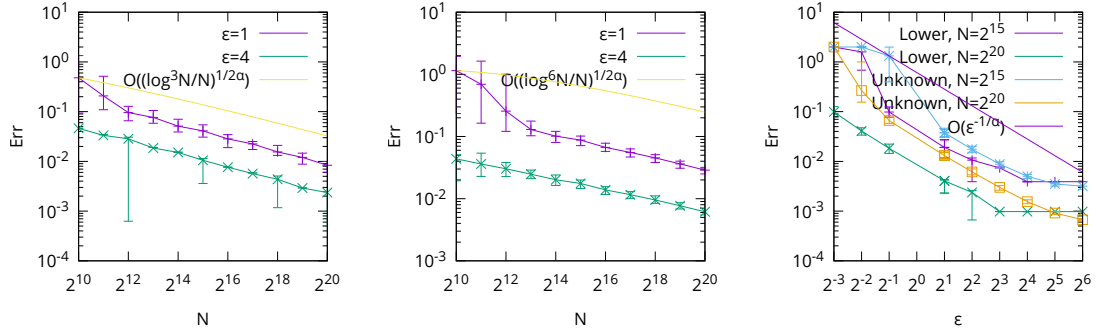

Figure 40: ( $\alpha = 0.9, \beta = 2, \Delta = 0.3$ , iid) Err v.s.  $N$  (left and middle) and Err v.s.  $\epsilon$  (right). The left figure depicts the result with **Lower**  $\alpha$ , and the middle figure depicts the result with **Unknown**  $\alpha$ .

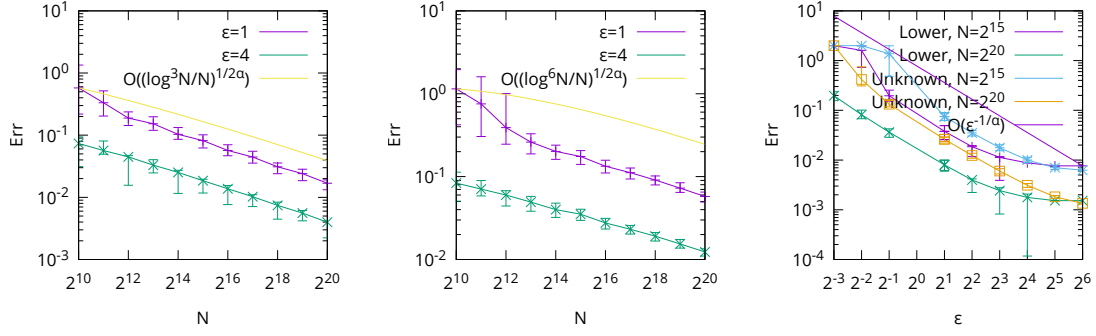

Figure 41: ( $\alpha = 0.9, \beta = 2, \Delta = 0.6$ , iid) Err v.s.  $N$  (left and middle) and Err v.s.  $\epsilon$  (right). The left figure depicts the result with **Lower**  $\alpha$ , and the middle figure depicts the result with **Unknown**  $\alpha$ .

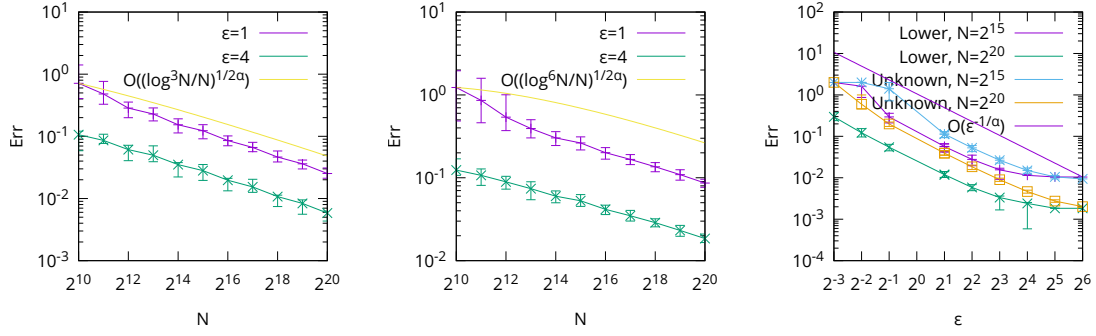

Figure 42: ( $\alpha = 0.9, \beta = 2, \Delta = 0.9$ , iid) Err v.s.  $N$  (left and middle) and Err v.s.  $\epsilon$  (right). The left figure depicts the result with **Lower**  $\alpha$ , and the middle figure depicts the result with **Unknown**  $\alpha$ .

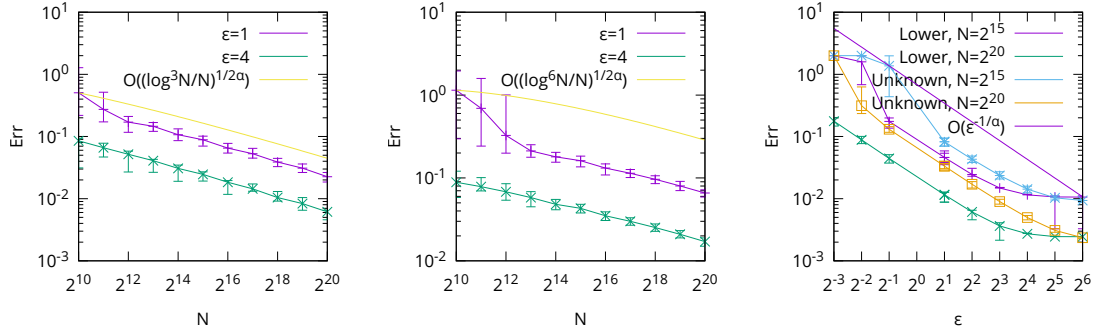

Figure 43: ( $\alpha = 1, \beta = 1, \Delta = 0.3$ , iid) Err v.s.  $N$  (left and middle) and Err v.s.  $\epsilon$  (right). The left figure depicts the result with **Lower**  $\alpha$ , and the middle figure depicts the result with **Unknown**  $\alpha$ .

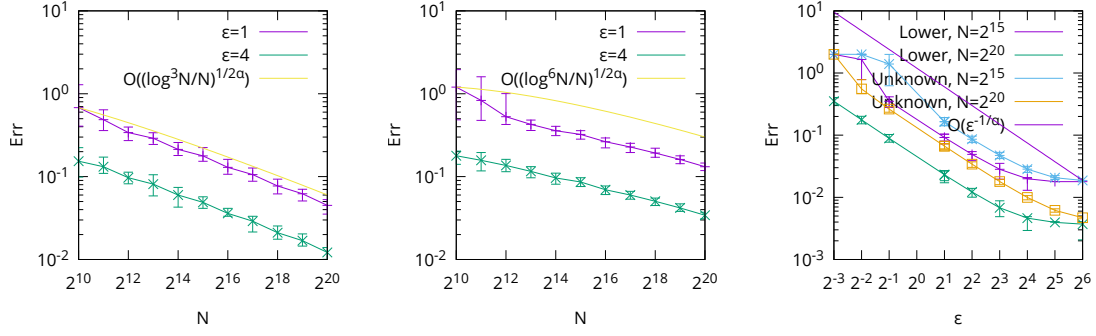

Figure 44: ( $\alpha = 1, \beta = 1, \Delta = 0.6$ , iid) Err v.s.  $N$  (left and middle) and Err v.s.  $\epsilon$  (right). The left figure depicts the result with **Lower**  $\alpha$ , and the middle figure depicts the result with **Unknown**  $\alpha$ .

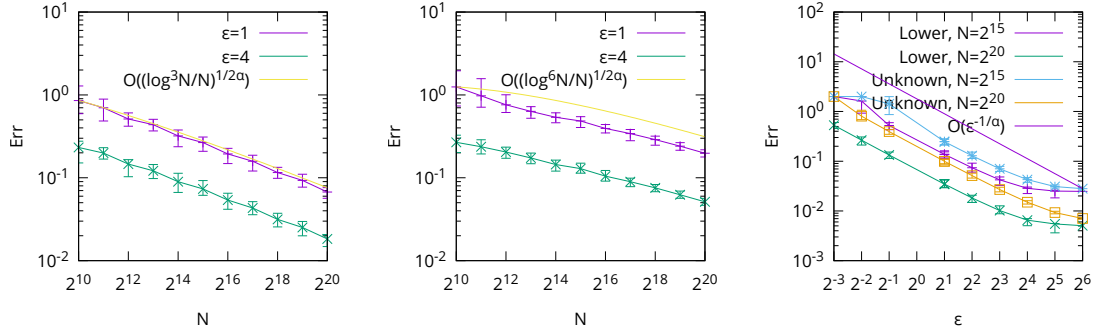

Figure 45: ( $\alpha = 1, \beta = 1, \Delta = 0.9$ , iid) Err v.s.  $N$  (left and middle) and Err v.s.  $\epsilon$  (right). The left figure depicts the result with **Lower**  $\alpha$ , and the middle figure depicts the result with **Unknown**  $\alpha$ .

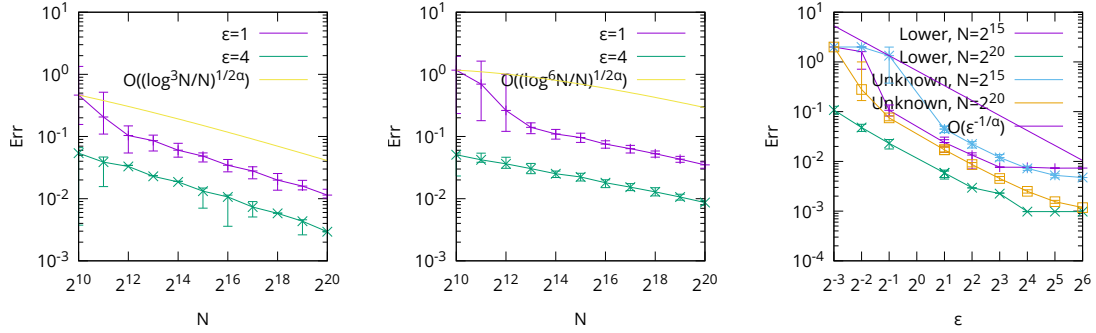

Figure 46: ( $\alpha = 1, \beta = 2, \Delta = 0.3$ , iid) Err v.s.  $N$  (left and middle) and Err v.s.  $\epsilon$  (right). The left figure depicts the result with **Lower**  $\alpha$ , and the middle figure depicts the result with **Unknown**  $\alpha$ .



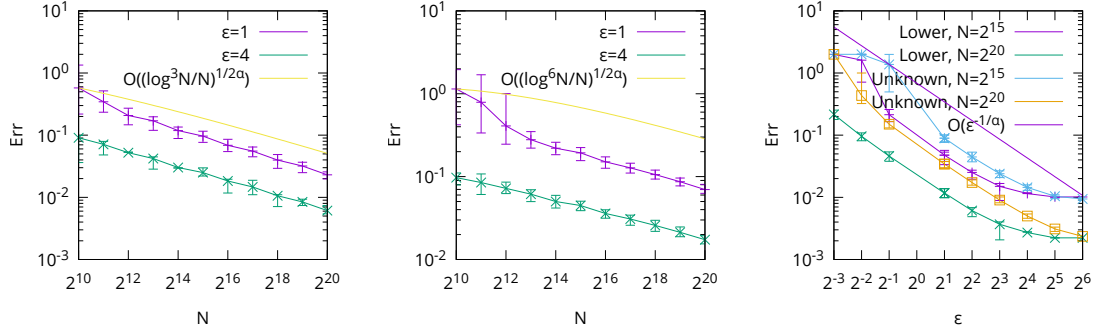

Figure 47: ( $\alpha = 1$ ,  $\beta = 2$ ,  $\Delta = 0.6$ , iid) Err v.s.  $N$  (left and middle) and Err v.s.  $\epsilon$  (right). The left figure depicts the result with **Lower**  $\alpha$ , and the middle figure depicts the result with **Unknown**  $\alpha$ .

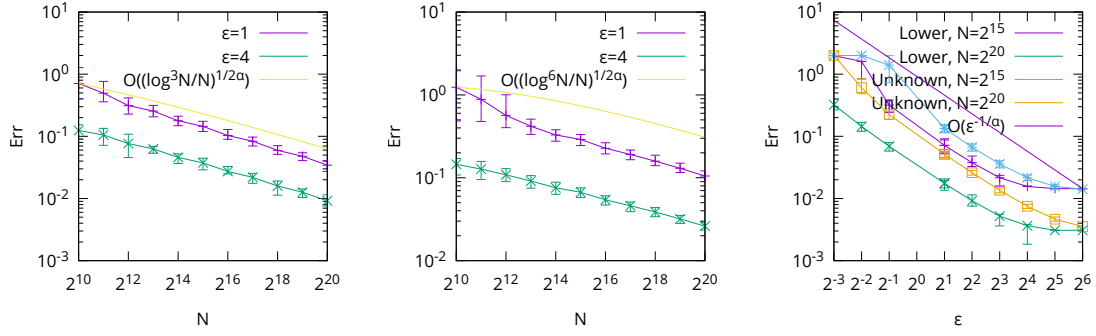

Figure 48: ( $\alpha = 1$ ,  $\beta = 2$ ,  $\Delta = 0.9$ , iid) Err v.s.  $N$  (left and middle) and Err v.s.  $\epsilon$  (right). The left figure depicts the result with **Lower**  $\alpha$ , and the middle figure depicts the result with **Unknown**  $\alpha$ .

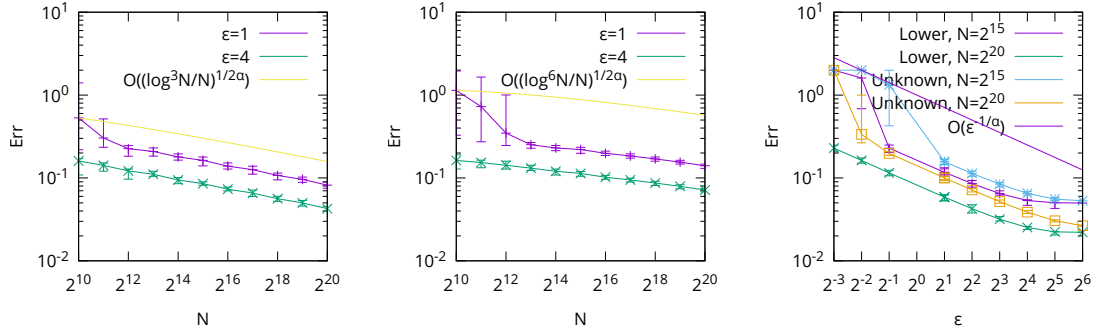

Figure 49: ( $\alpha = 2$ ,  $\beta = 1$ ,  $\Delta = 0.3$ , iid) Err v.s.  $N$  (left and middle) and Err v.s.  $\epsilon$  (right). The left figure depicts the result with **Lower**  $\alpha$ , and the middle figure depicts the result with **Unknown**  $\alpha$ .

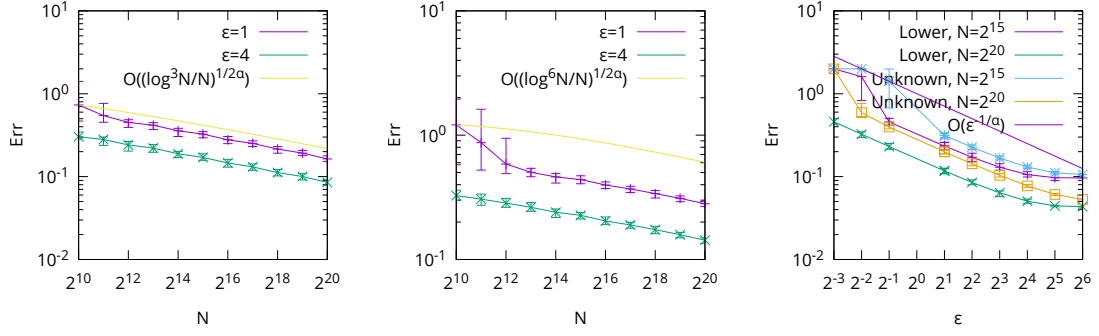

Figure 50: ( $\alpha = 2$ ,  $\beta = 1$ ,  $\Delta = 0.6$ , iid) Err v.s.  $N$  (left and middle) and Err v.s.  $\epsilon$  (right). The left figure depicts the result with **Lower**  $\alpha$ , and the middle figure depicts the result with **Unknown**  $\alpha$ .

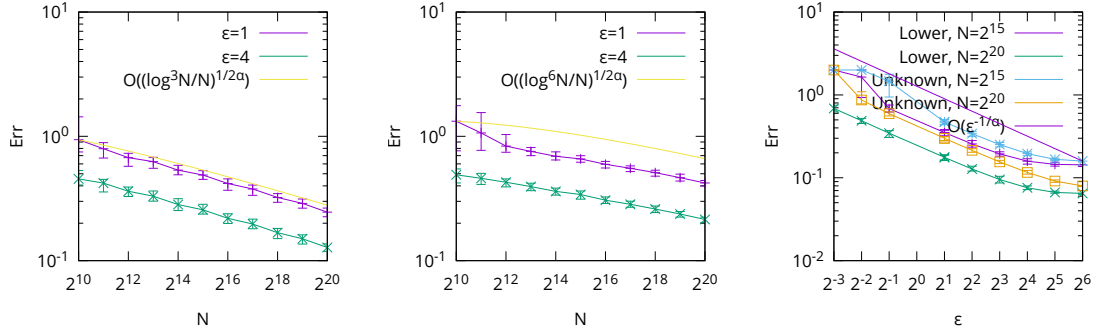

Figure 51: ( $\alpha = 2$ ,  $\beta = 1$ ,  $\Delta = 0.9$ , iid) Err v.s.  $N$  (left and middle) and Err v.s.  $\epsilon$  (right). The left figure depicts the result with **Lower**  $\alpha$ , and the middle figure depicts the result with **Unknown**  $\alpha$ .

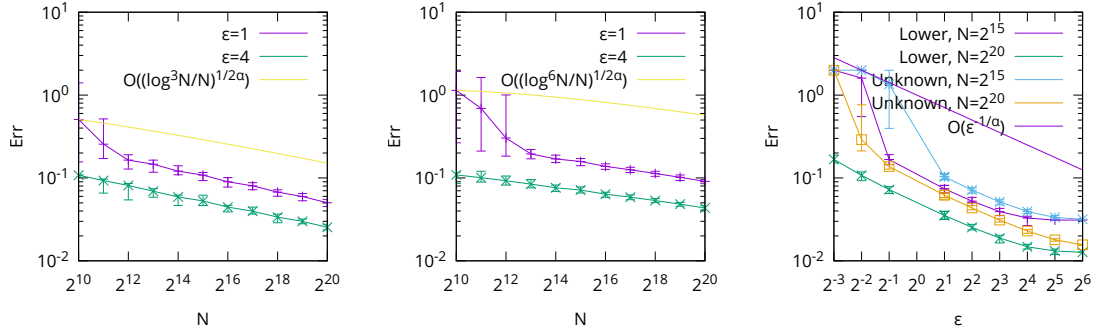

Figure 52: ( $\alpha = 2$ ,  $\beta = 2$ ,  $\Delta = 0.3$ , iid) Err v.s.  $N$  (left and middle) and Err v.s.  $\epsilon$  (right). The left figure depicts the result with **Lower**  $\alpha$ , and the middle figure depicts the result with **Unknown**  $\alpha$ .

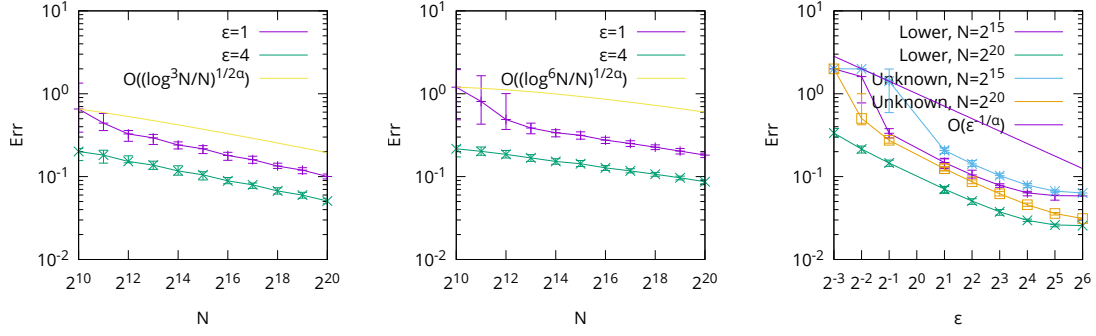

Figure 53: ( $\alpha = 2, \beta = 2, \Delta = 0.6$ , iid) Err v.s.  $N$  (left and middle) and Err v.s.  $\epsilon$  (right). The left figure depicts the result with **Lower**  $\alpha$ , and the middle figure depicts the result with **Unknown**  $\alpha$ .

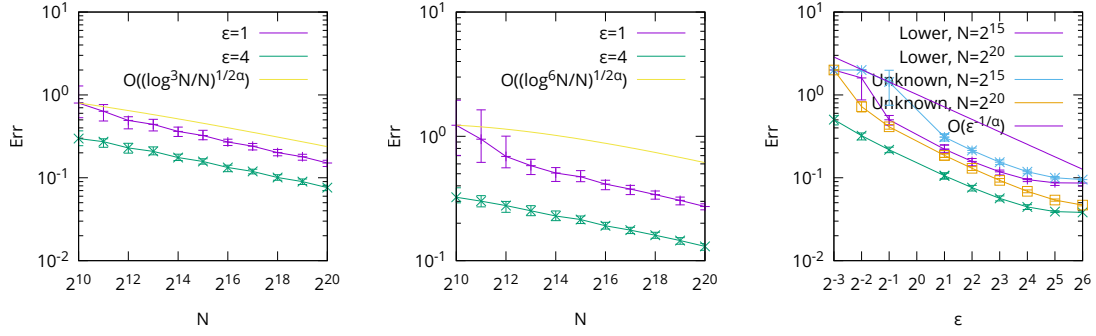

Figure 54: ( $\alpha = 2, \beta = 2, \Delta = 0.9$ , iid) Err v.s.  $N$  (left and middle) and Err v.s.  $\epsilon$  (right). The left figure depicts the result with **Lower**  $\alpha$ , and the middle figure depicts the result with **Unknown**  $\alpha$ .

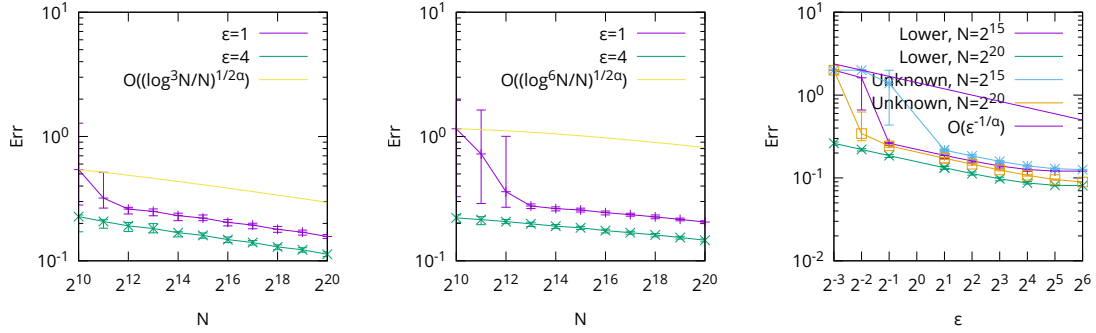

Figure 55: ( $\alpha = 4, \beta = 1, \Delta = 0.3$ , iid) Err v.s.  $N$  (left and middle) and Err v.s.  $\epsilon$  (right). The left figure depicts the result with **Lower**  $\alpha$ , and the middle figure depicts the result with **Unknown**  $\alpha$ .

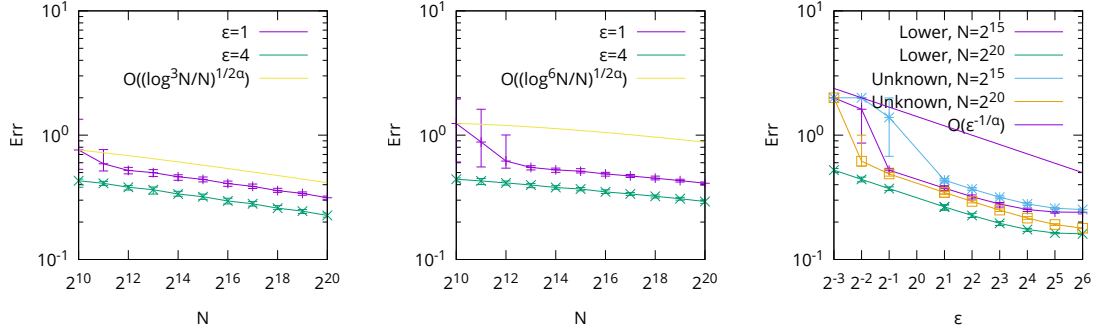

Figure 56: ( $\alpha = 4, \beta = 1, \Delta = 0.6$ , iid) Err v.s.  $N$  (left and middle) and Err v.s.  $\epsilon$  (right). The left figure depicts the result with **Lower**  $\alpha$ , and the middle figure depicts the result with **Unknown**  $\alpha$ .

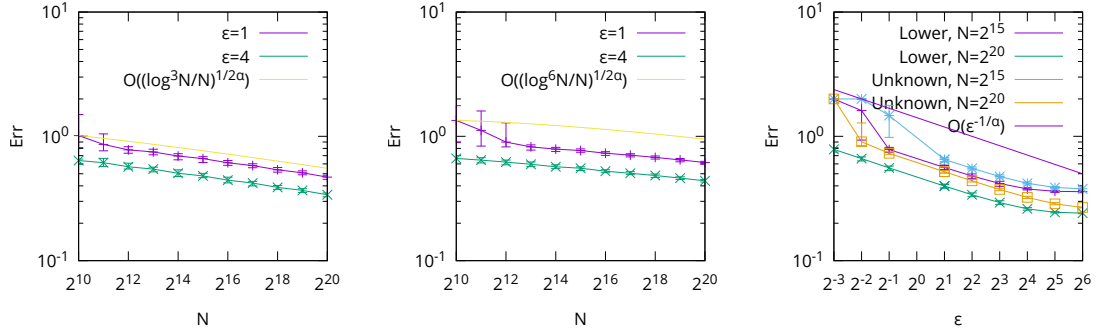

Figure 57: ( $\alpha = 4, \beta = 1, \Delta = 0.9$ , iid) Err v.s.  $N$  (left and middle) and Err v.s.  $\epsilon$  (right). The left figure depicts the result with **Lower**  $\alpha$ , and the middle figure depicts the result with **Unknown**  $\alpha$ .

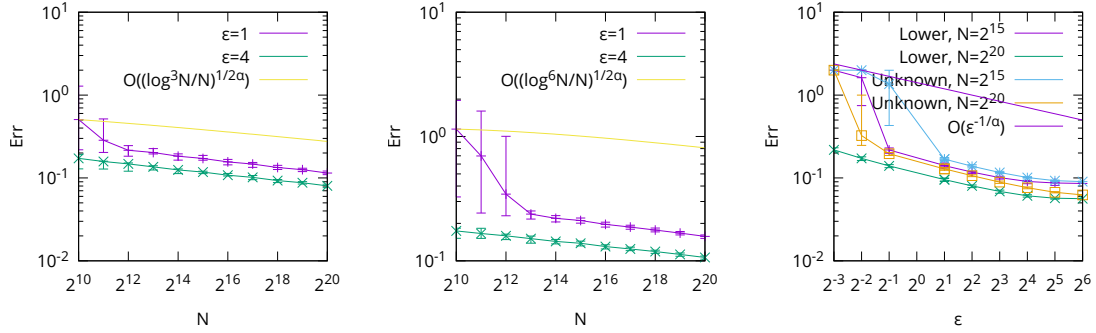

Figure 58: ( $\alpha = 4, \beta = 2, \Delta = 0.3$ , iid) Err v.s.  $N$  (left and middle) and Err v.s.  $\epsilon$  (right). The left figure depicts the result with **Lower**  $\alpha$ , and the middle figure depicts the result with **Unknown**  $\alpha$ .

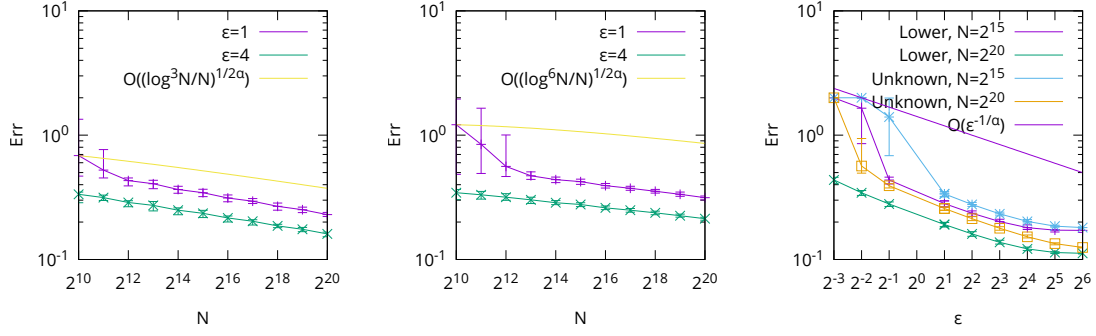

Figure 59: ( $\alpha = 4$ ,  $\beta = 2$ ,  $\Delta = 0.6$ , iid) Err v.s.  $N$  (left and middle) and Err v.s.  $\epsilon$  (right). The left figure depicts the result with **Lower**  $\alpha$ , and the middle figure depicts the result with **Unknown**  $\alpha$ .

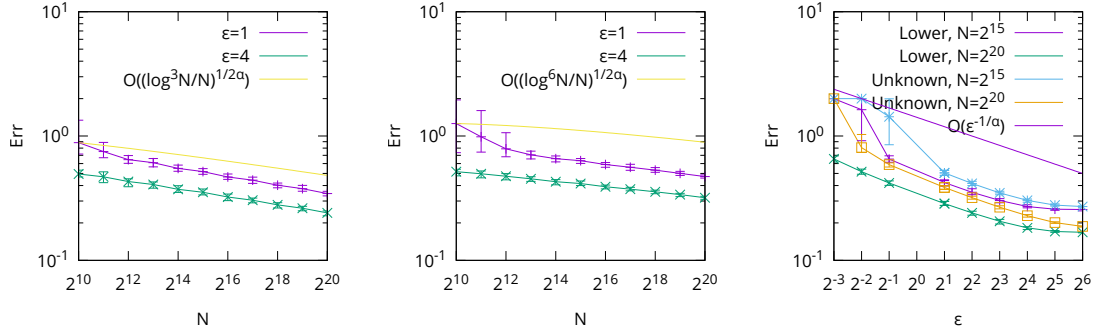

Figure 60: ( $\alpha = 4$ ,  $\beta = 2$ ,  $\Delta = 0.9$ , iid) Err v.s.  $N$  (left and middle) and Err v.s.  $\epsilon$  (right). The left figure depicts the result with **Lower**  $\alpha$ , and the middle figure depicts the result with **Unknown**  $\alpha$ .

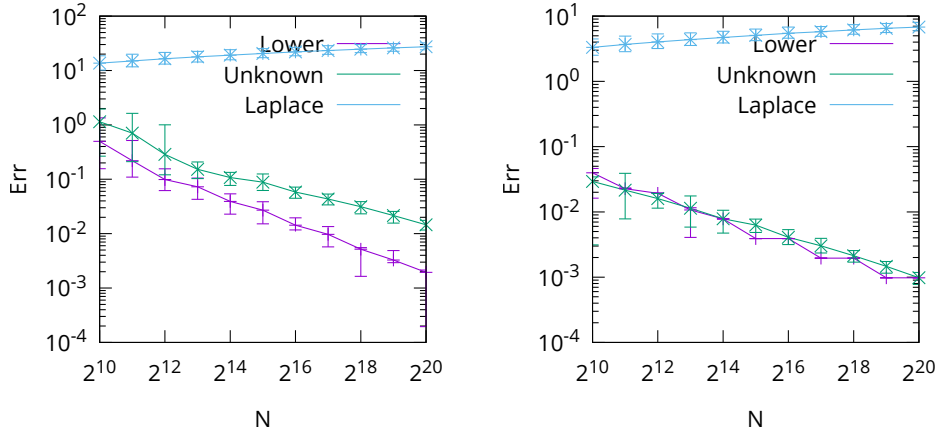

Figure 61: ( $\alpha = 0.5$ ,  $\beta = 1$ ,  $\Delta = 0.3$ , fixed) Comparison between our methods and the baseline method with  $\epsilon = 1$  (left) and  $\epsilon = 4$  (right).

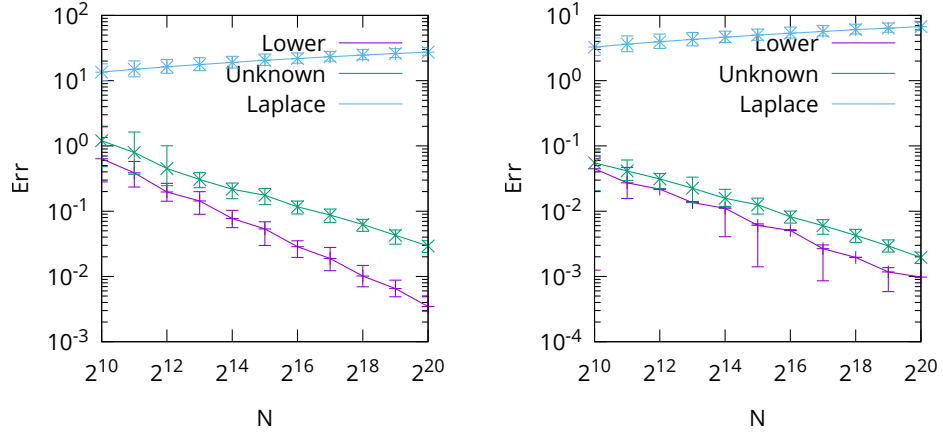

Figure 62: ( $\alpha = 0.5$ ,  $\beta = 1$ ,  $\Delta = 0.6$ , fixed) Comparison between our methods and the baseline method with  $\epsilon = 1$  (left) and  $\epsilon = 4$  (right).

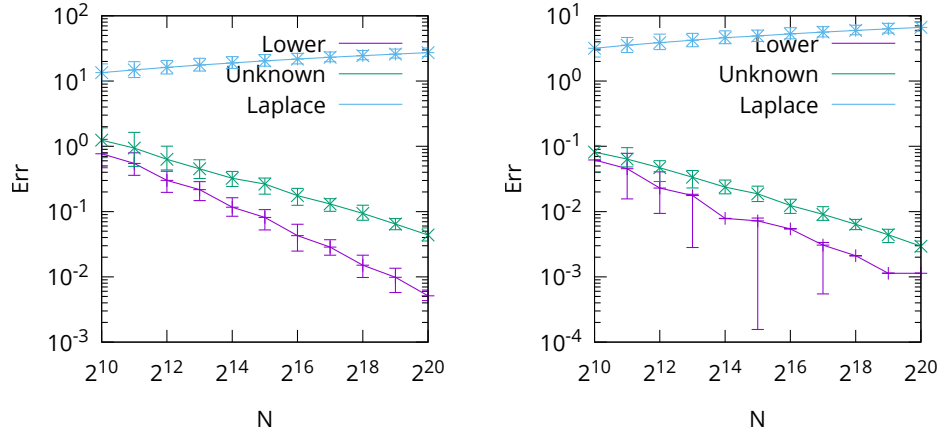

Figure 63: ( $\alpha = 0.5$ ,  $\beta = 1$ ,  $\Delta = 0.9$ , fixed) Comparison between our methods and the baseline method with  $\epsilon = 1$  (left) and  $\epsilon = 4$  (right).

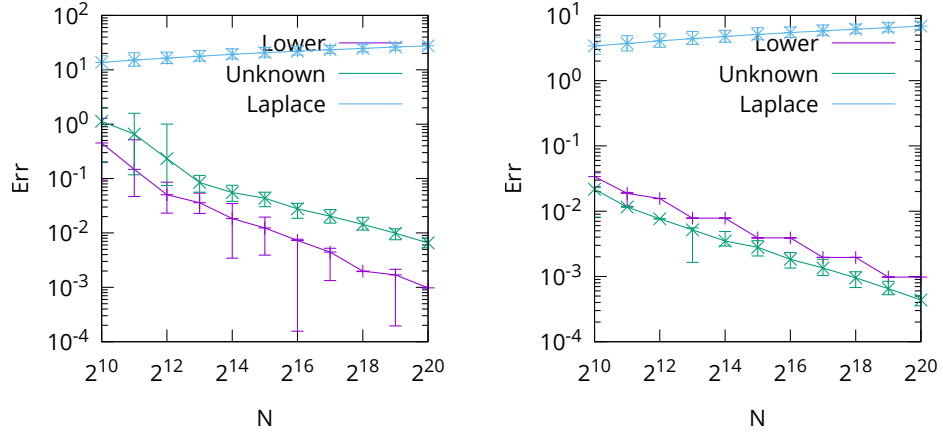

Figure 64: ( $\alpha = 0.5$ ,  $\beta = 2$ ,  $\Delta = 0.3$ , fixed) Comparison between our methods and the baseline method with  $\epsilon = 1$  (left) and  $\epsilon = 4$  (right).

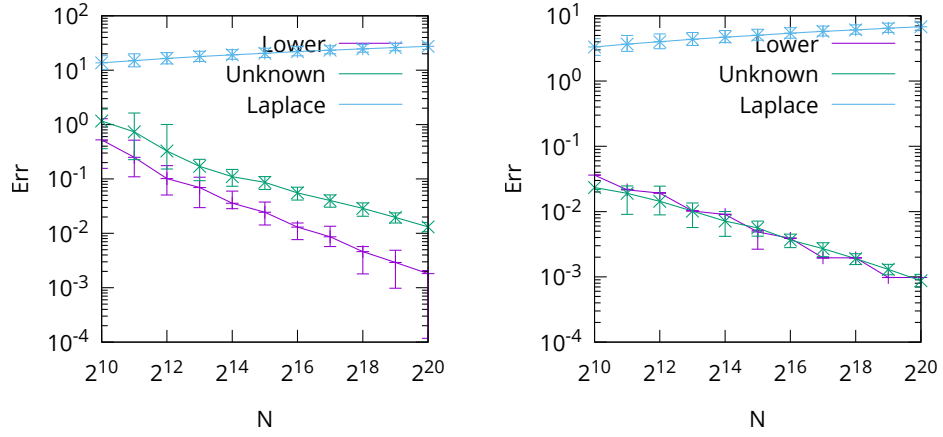

Figure 65: ( $\alpha = 0.5$ ,  $\beta = 2$ ,  $\Delta = 0.6$ , fixed) Comparison between our methods and the baseline method with  $\epsilon = 1$  (left) and  $\epsilon = 4$  (right).

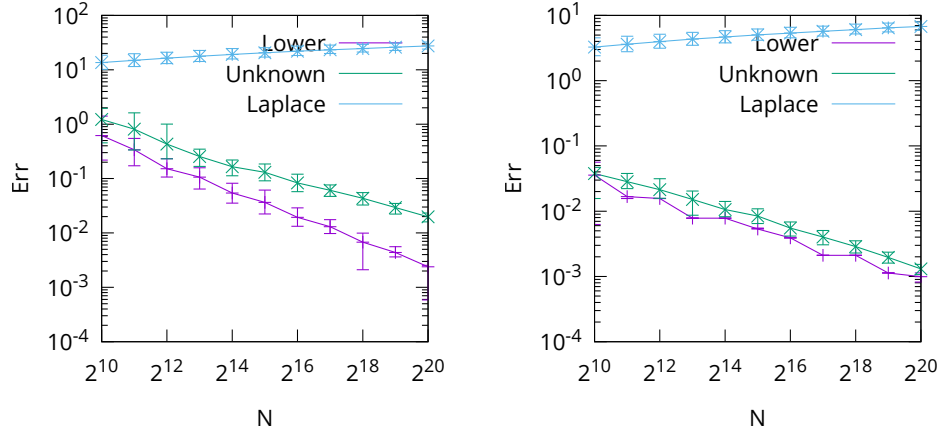

Figure 66: ( $\alpha = 0.5$ ,  $\beta = 2$ ,  $\Delta = 0.9$ , fixed) Comparison between our methods and the baseline method with  $\epsilon = 1$  (left) and  $\epsilon = 4$  (right).

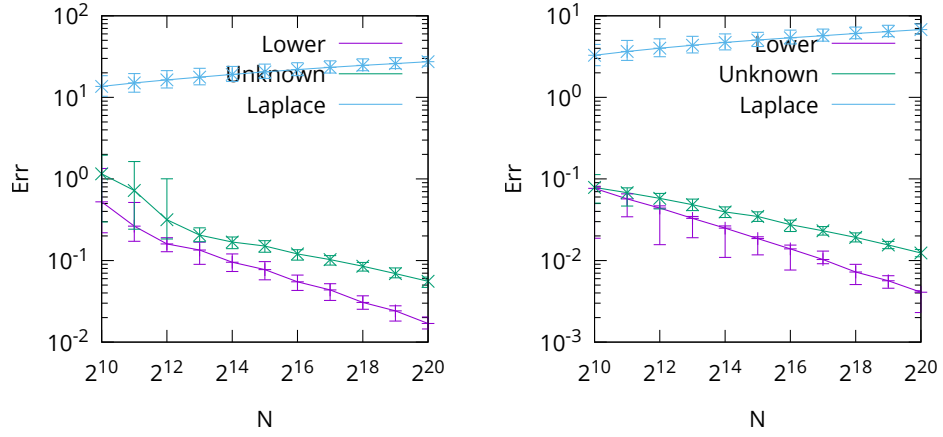

Figure 67: ( $\alpha = 0.9$ ,  $\beta = 1$ ,  $\Delta = 0.3$ , fixed) Comparison between our methods and the baseline method with  $\epsilon = 1$  (left) and  $\epsilon = 4$  (right).



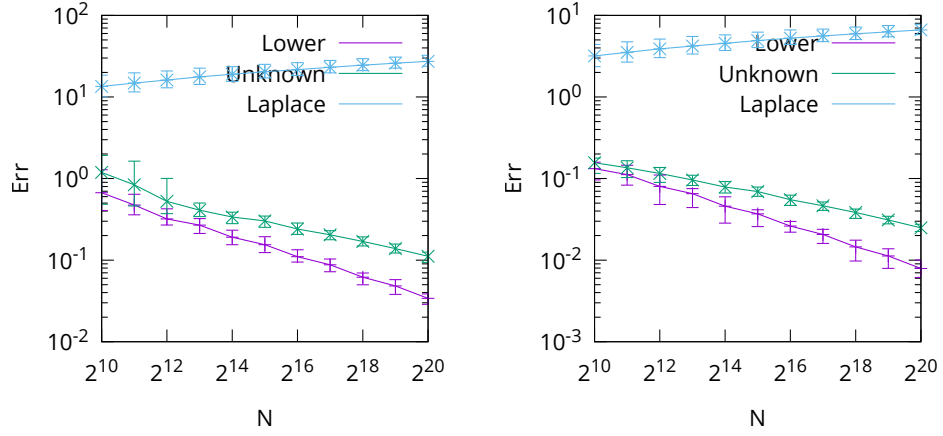

Figure 68: ( $\alpha = 0.9$ ,  $\beta = 1$ ,  $\Delta = 0.6$ , fixed) Comparison between our methods and the baseline method with  $\epsilon = 1$  (left) and  $\epsilon = 4$  (right).

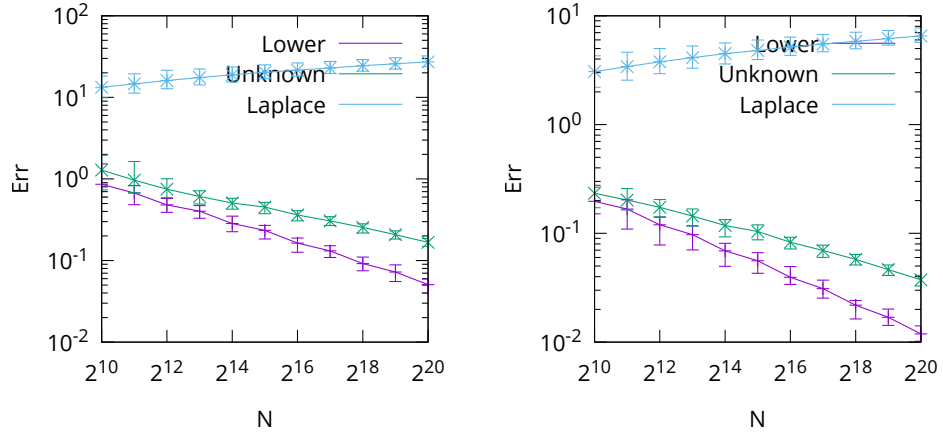

Figure 69: ( $\alpha = 0.9$ ,  $\beta = 1$ ,  $\Delta = 0.9$ , fixed) Comparison between our methods and the baseline method with  $\epsilon = 1$  (left) and  $\epsilon = 4$  (right).

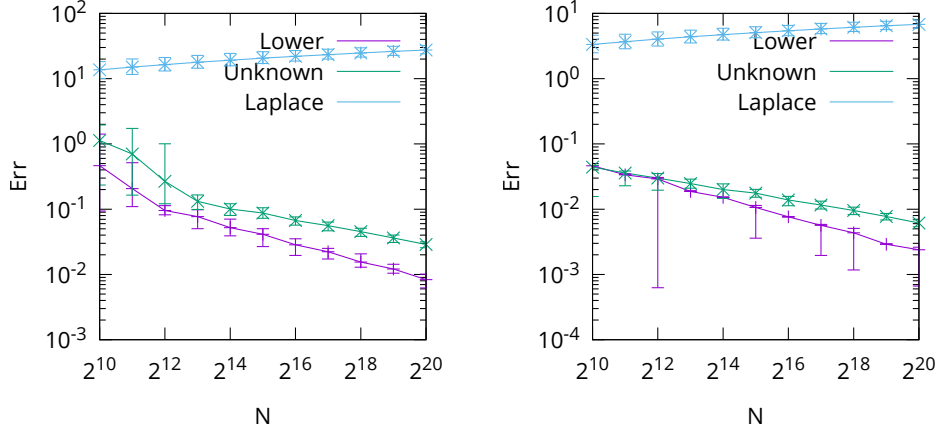

Figure 70: ( $\alpha = 0.9$ ,  $\beta = 2$ ,  $\Delta = 0.3$ , fixed) Comparison between our methods and the baseline method with  $\epsilon = 1$  (left) and  $\epsilon = 4$  (right).

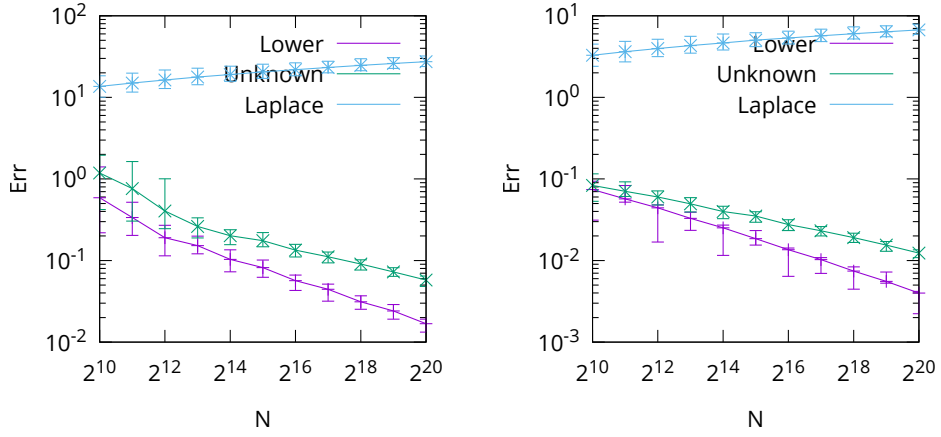

Figure 71: ( $\alpha = 0.9$ ,  $\beta = 2$ ,  $\Delta = 0.6$ , fixed) Comparison between our methods and the baseline method with  $\epsilon = 1$  (left) and  $\epsilon = 4$  (right).

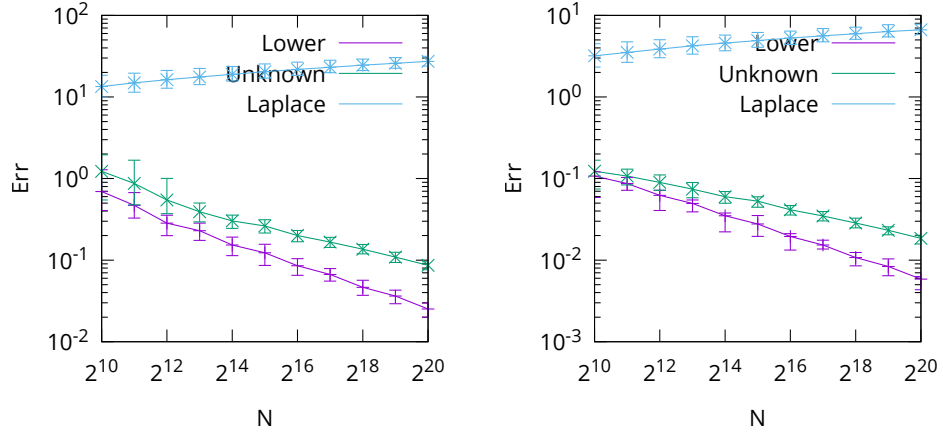

Figure 72: ( $\alpha = 0.9$ ,  $\beta = 2$ ,  $\Delta = 0.9$ , fixed) Comparison between our methods and the baseline method with  $\epsilon = 1$  (left) and  $\epsilon = 4$  (right).

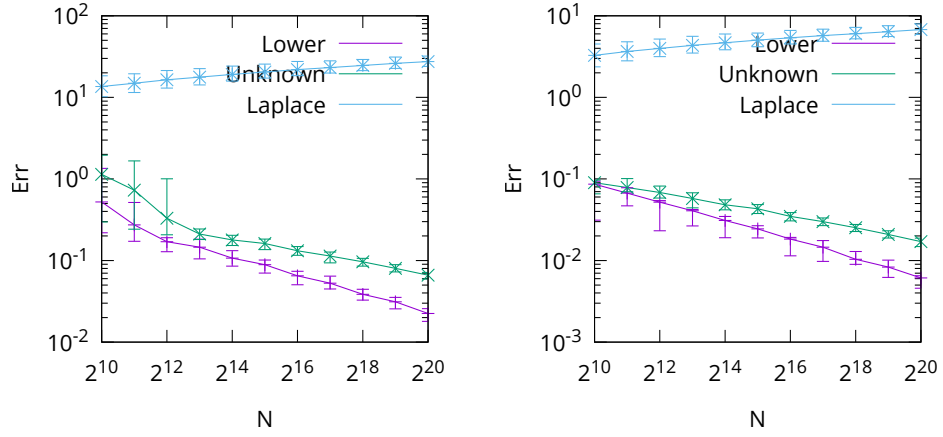

Figure 73: ( $\alpha = 1$ ,  $\beta = 1$ ,  $\Delta = 0.3$ , fixed) Comparison between our methods and the baseline method with  $\epsilon = 1$  (left) and  $\epsilon = 4$  (right).

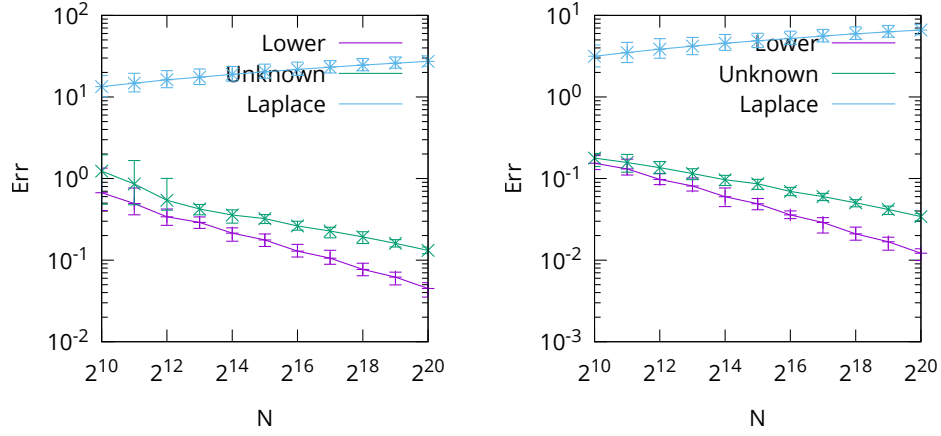

Figure 74: ( $\alpha = 1, \beta = 1, \Delta = 0.6$ , fixed) Comparison between our methods and the baseline method with  $\epsilon = 1$  (left) and  $\epsilon = 4$  (right).

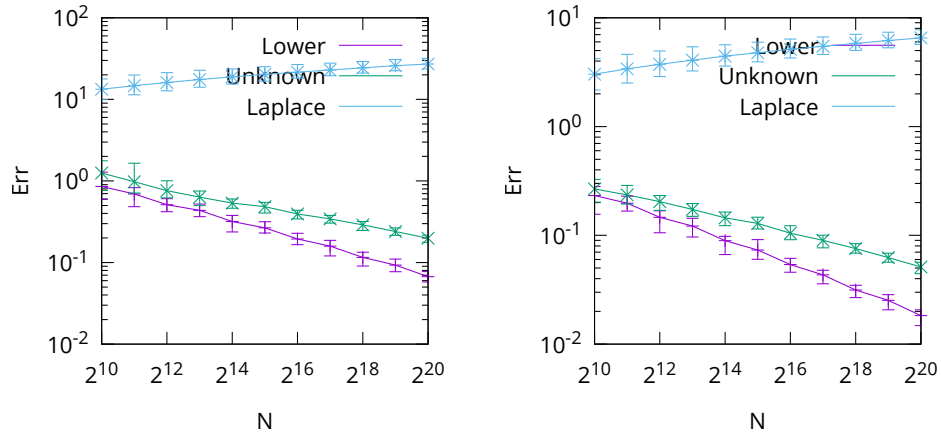

Figure 75: ( $\alpha = 1, \beta = 1, \Delta = 0.9$ , fixed) Comparison between our methods and the baseline method with  $\epsilon = 1$  (left) and  $\epsilon = 4$  (right).

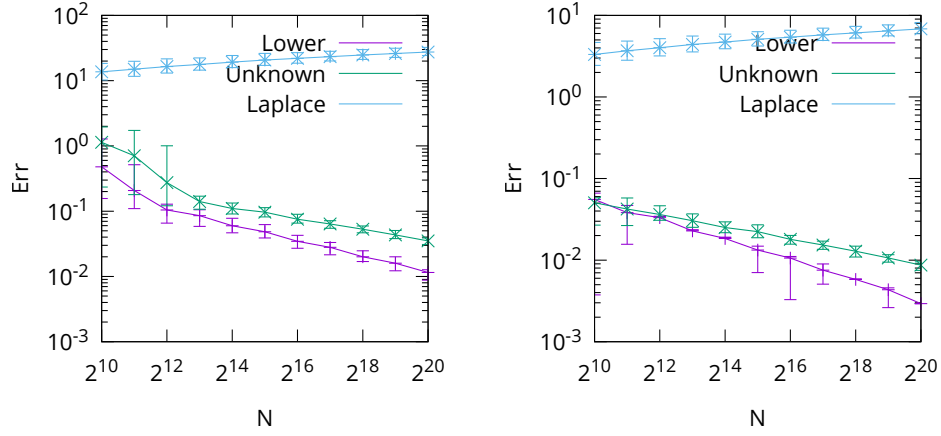

Figure 76: ( $\alpha = 1$ ,  $\beta = 2$ ,  $\Delta = 0.3$ , fixed) Comparison between our methods and the baseline method with  $\epsilon = 1$  (left) and  $\epsilon = 4$  (right).

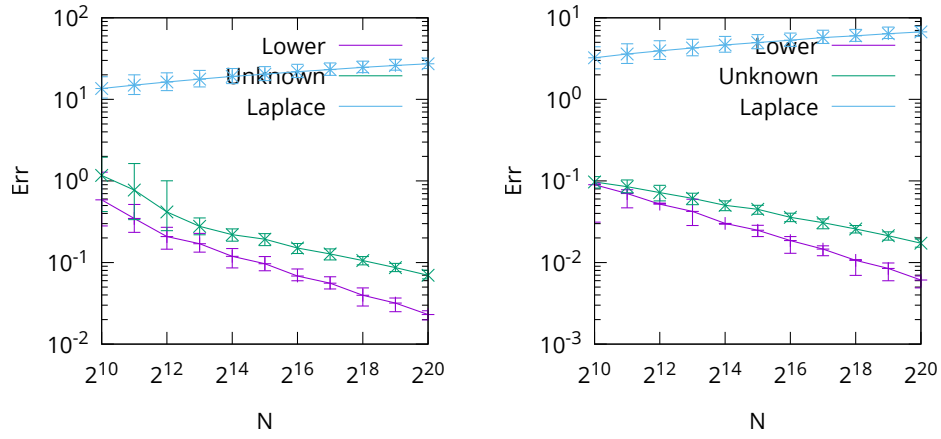

Figure 77: ( $\alpha = 1$ ,  $\beta = 2$ ,  $\Delta = 0.6$ , fixed) Comparison between our methods and the baseline method with  $\epsilon = 1$  (left) and  $\epsilon = 4$  (right).

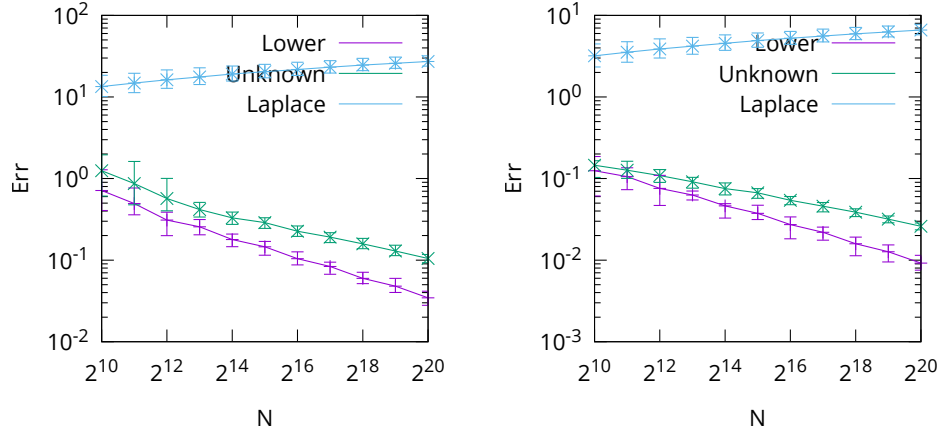

Figure 78: ( $\alpha = 1$ ,  $\beta = 2$ ,  $\Delta = 0.9$ , fixed) Comparison between our methods and the baseline method with  $\epsilon = 1$  (left) and  $\epsilon = 4$  (right).

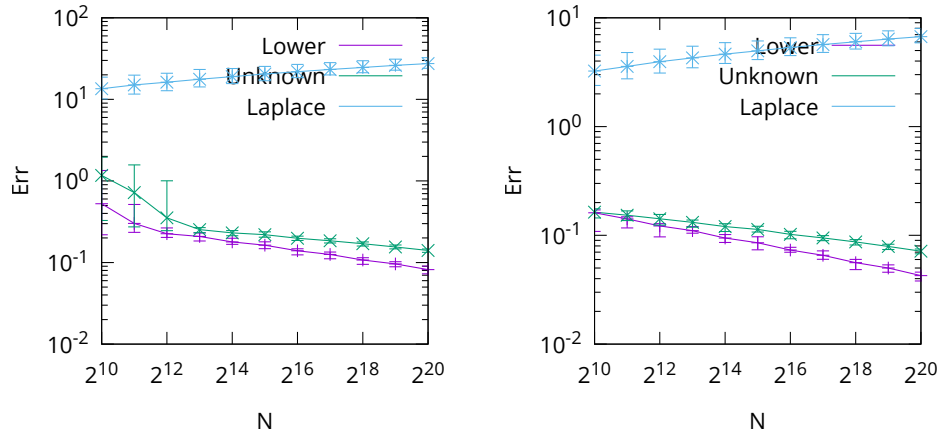

Figure 79: ( $\alpha = 2$ ,  $\beta = 1$ ,  $\Delta = 0.3$ , fixed) Comparison between our methods and the baseline method with  $\epsilon = 1$  (left) and  $\epsilon = 4$  (right).

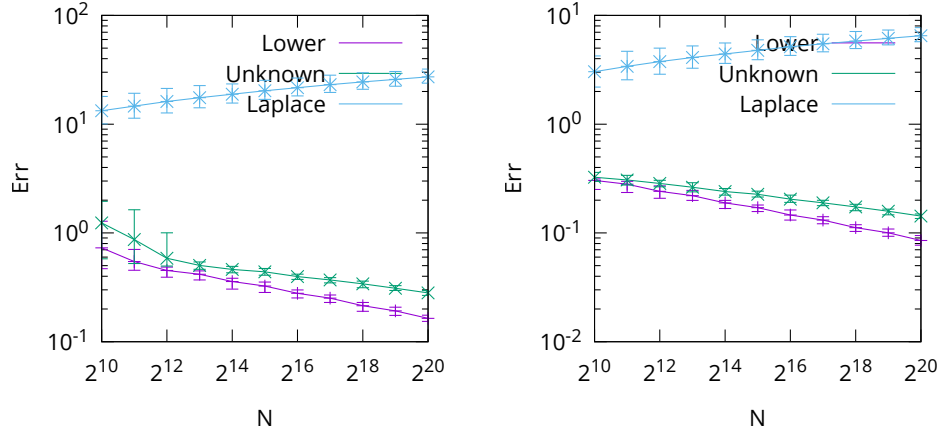

Figure 80: ( $\alpha = 2$ ,  $\beta = 1$ ,  $\Delta = 0.6$ , fixed) Comparison between our methods and the baseline method with  $\epsilon = 1$  (left) and  $\epsilon = 4$  (right).

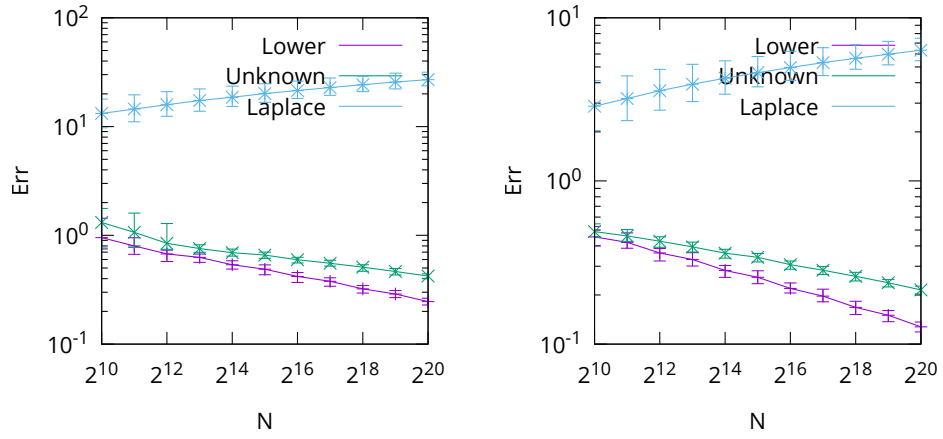

Figure 81: ( $\alpha = 2$ ,  $\beta = 1$ ,  $\Delta = 0.9$ , fixed) Comparison between our methods and the baseline method with  $\epsilon = 1$  (left) and  $\epsilon = 4$  (right).

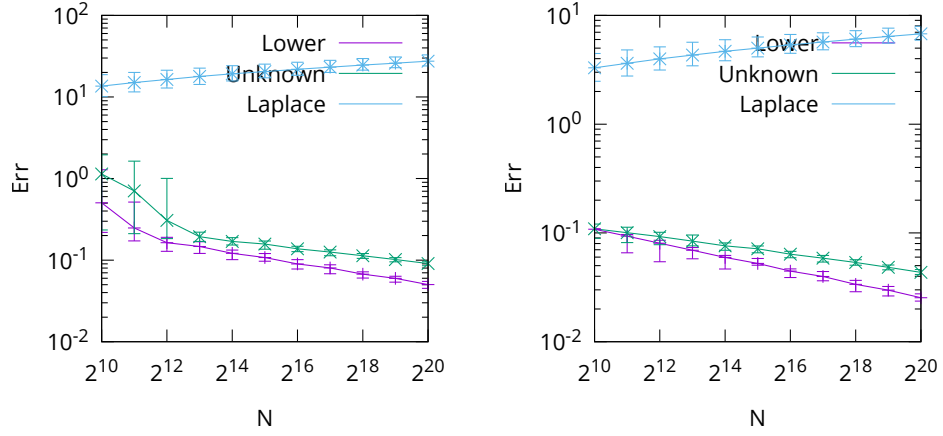

Figure 82: ( $\alpha = 2, \beta = 2, \Delta = 0.3$ , fixed) Comparison between our methods and the baseline method with  $\epsilon = 1$  (left) and  $\epsilon = 4$  (right).

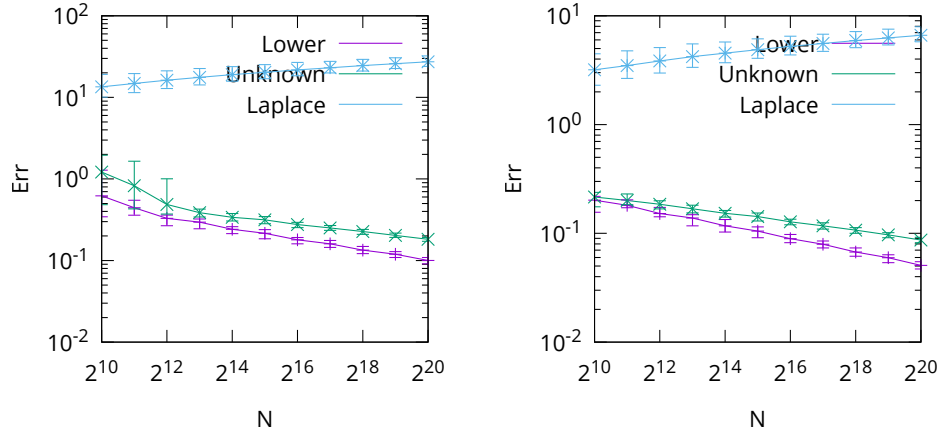

Figure 83: ( $\alpha = 2, \beta = 2, \Delta = 0.6$ , fixed) Comparison between our methods and the baseline method with  $\epsilon = 1$  (left) and  $\epsilon = 4$  (right).



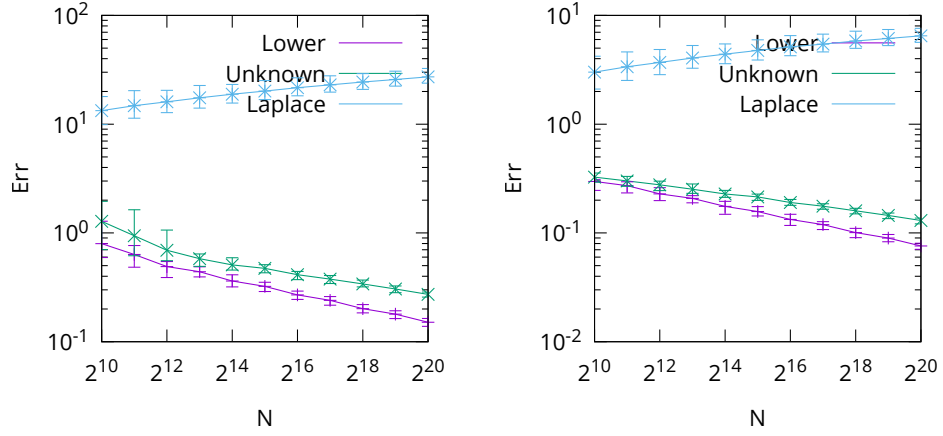

Figure 84: ( $\alpha = 2$ ,  $\beta = 2$ ,  $\Delta = 0.9$ , fixed) Comparison between our methods and the baseline method with  $\epsilon = 1$  (left) and  $\epsilon = 4$  (right).

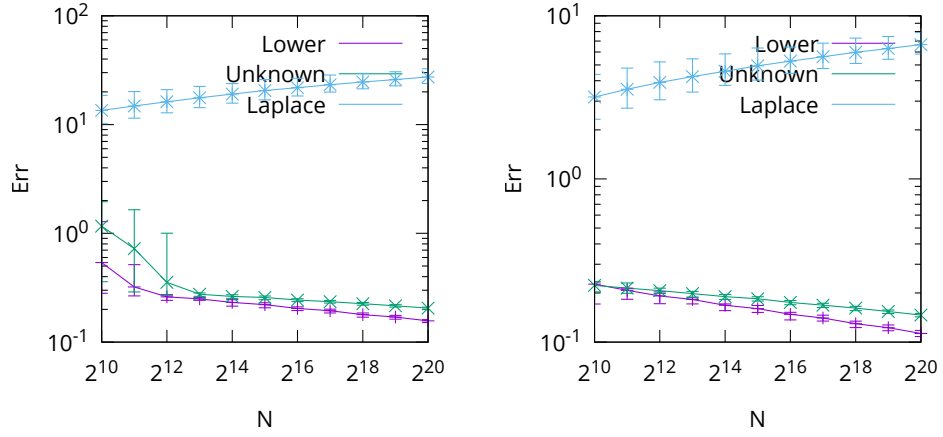

Figure 85: ( $\alpha = 4$ ,  $\beta = 1$ ,  $\Delta = 0.3$ , fixed) Comparison between our methods and the baseline method with  $\epsilon = 1$  (left) and  $\epsilon = 4$  (right).

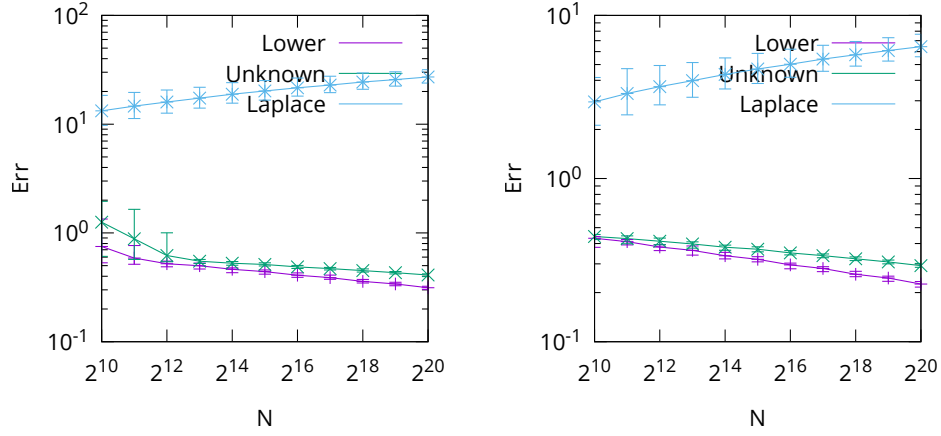

Figure 86: ( $\alpha = 4, \beta = 1, \Delta = 0.6$ , fixed) Comparison between our methods and the baseline method with  $\epsilon = 1$  (left) and  $\epsilon = 4$  (right).

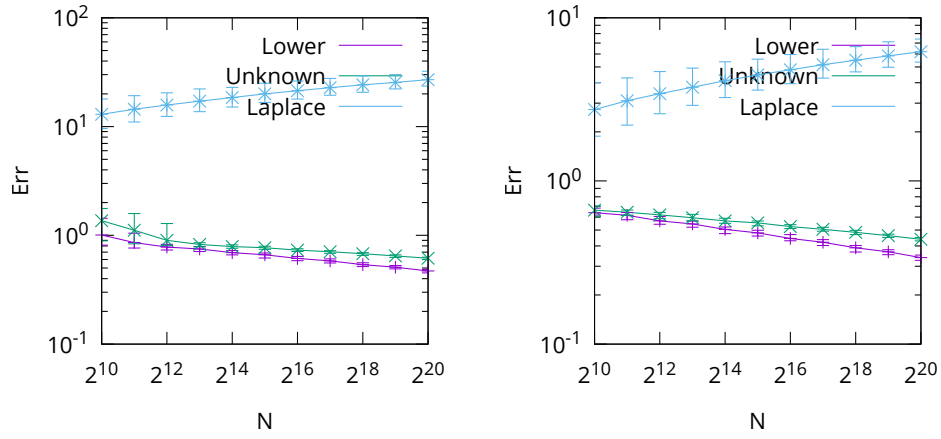

Figure 87: ( $\alpha = 4, \beta = 1, \Delta = 0.9$ , fixed) Comparison between our methods and the baseline method with  $\epsilon = 1$  (left) and  $\epsilon = 4$  (right).

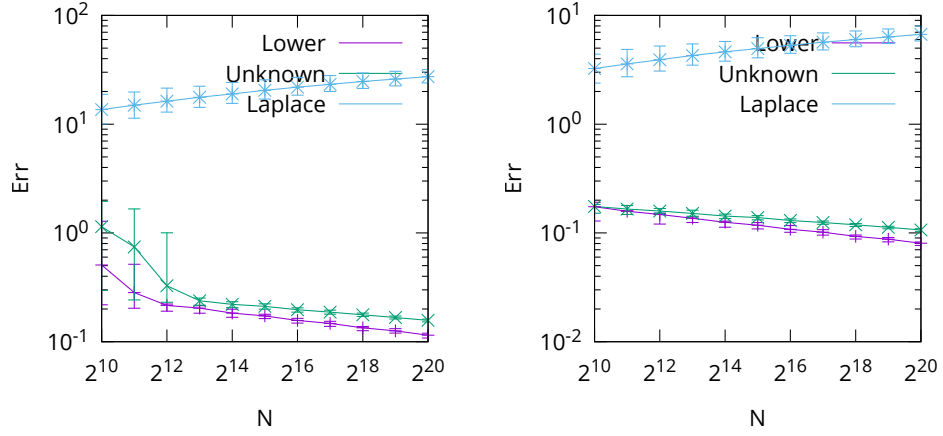

Figure 88: ( $\alpha = 4, \beta = 2, \Delta = 0.3$ , fixed) Comparison between our methods and the baseline method with  $\epsilon = 1$  (left) and  $\epsilon = 4$  (right).

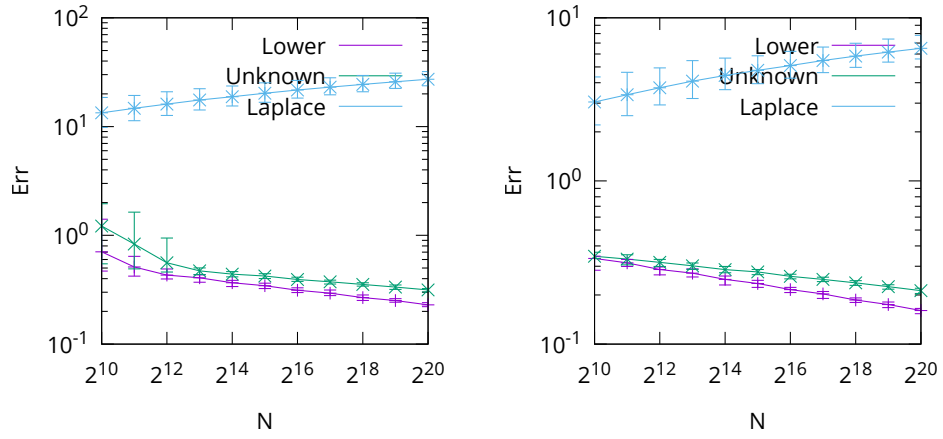

Figure 89: ( $\alpha = 4, \beta = 2, \Delta = 0.6$ , fixed) Comparison between our methods and the baseline method with  $\epsilon = 1$  (left) and  $\epsilon = 4$  (right).

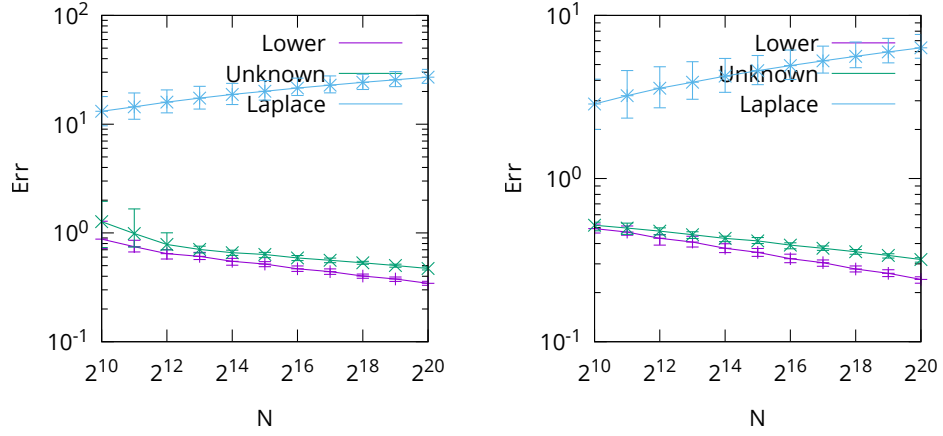

Figure 90: ( $\alpha = 4, \beta = 2, \Delta = 0.9$ , fixed) Comparison between our methods and the baseline method with  $\epsilon = 1$  (left) and  $\epsilon = 4$  (right).

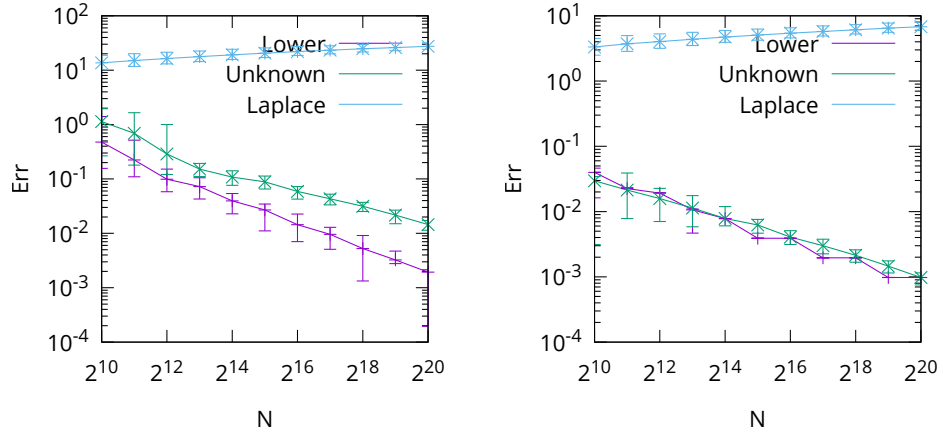

Figure 91: ( $\alpha = 0.5, \beta = 1, \Delta = 0.3$ , iid) Comparison between our methods and the baseline method with  $\epsilon = 1$  (left) and  $\epsilon = 4$  (right).

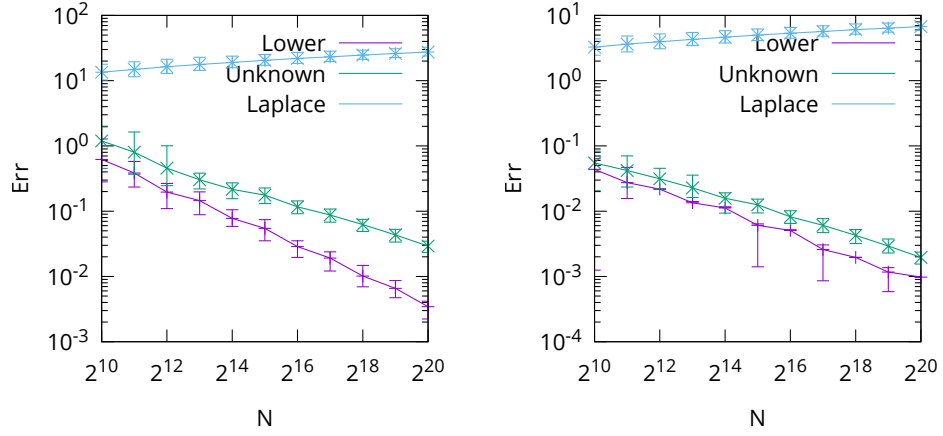

Figure 92: ( $\alpha = 0.5$ ,  $\beta = 1$ ,  $\Delta = 0.6$ , iid) Comparison between our methods and the baseline method with  $\epsilon = 1$  (left) and  $\epsilon = 4$  (right).

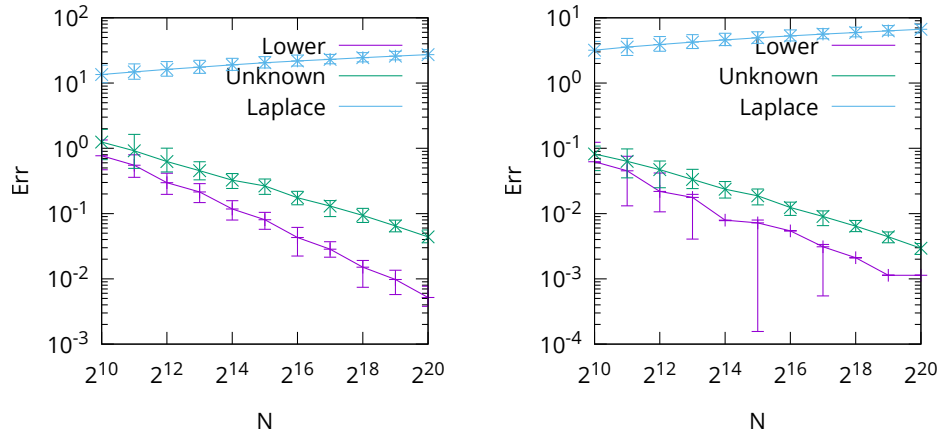

Figure 93: ( $\alpha = 0.5$ ,  $\beta = 1$ ,  $\Delta = 0.9$ , iid) Comparison between our methods and the baseline method with  $\epsilon = 1$  (left) and  $\epsilon = 4$  (right).

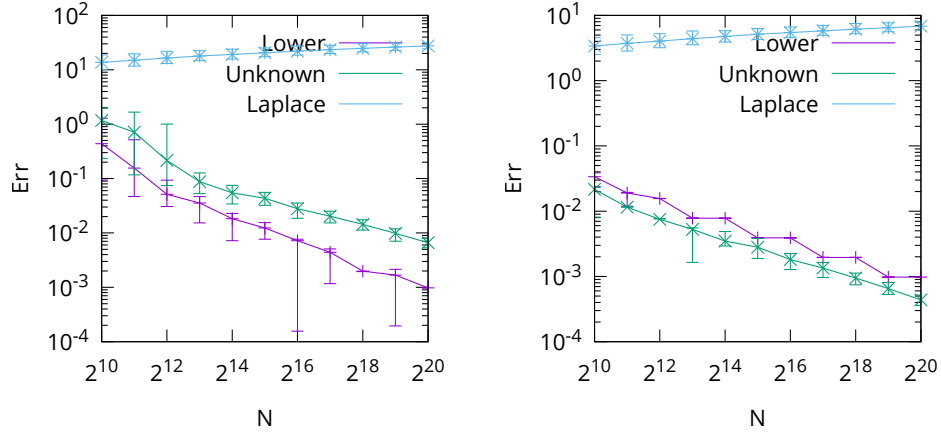

Figure 94: ( $\alpha = 0.5$ ,  $\beta = 2$ ,  $\Delta = 0.3$ , iid) Comparison between our methods and the baseline method with  $\epsilon = 1$  (left) and  $\epsilon = 4$  (right).

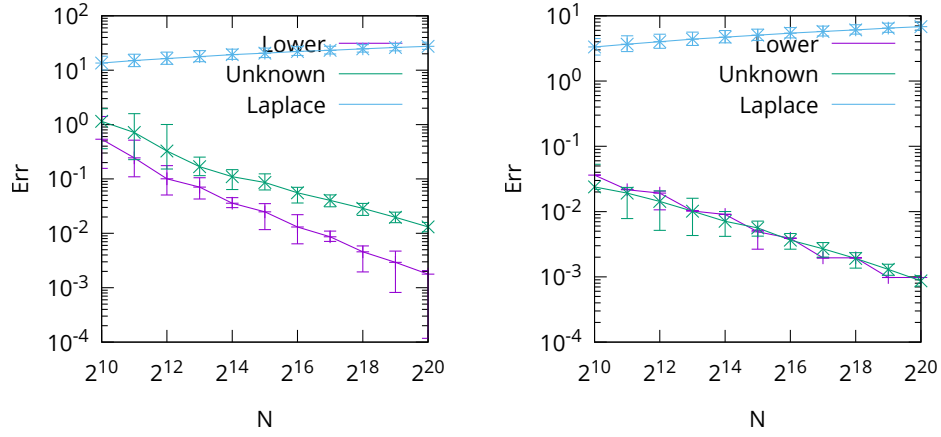

Figure 95: ( $\alpha = 0.5$ ,  $\beta = 2$ ,  $\Delta = 0.6$ , iid) Comparison between our methods and the baseline method with  $\epsilon = 1$  (left) and  $\epsilon = 4$  (right).

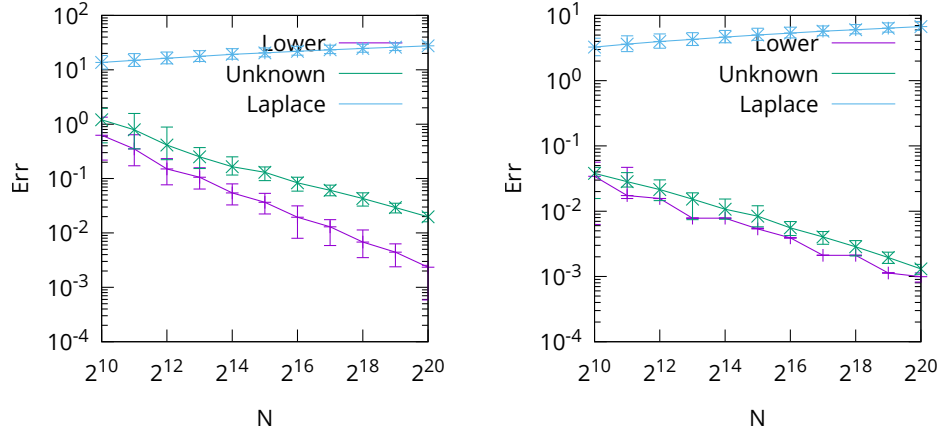

Figure 96: ( $\alpha = 0.5$ ,  $\beta = 2$ ,  $\Delta = 0.9$ , iid) Comparison between our methods and the baseline method with  $\epsilon = 1$  (left) and  $\epsilon = 4$  (right).

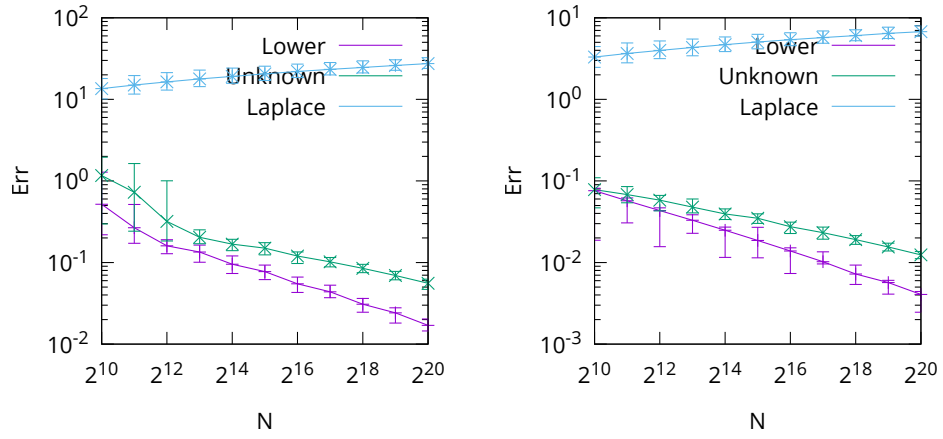

Figure 97: ( $\alpha = 0.9$ ,  $\beta = 1$ ,  $\Delta = 0.3$ , iid) Comparison between our methods and the baseline method with  $\epsilon = 1$  (left) and  $\epsilon = 4$  (right).

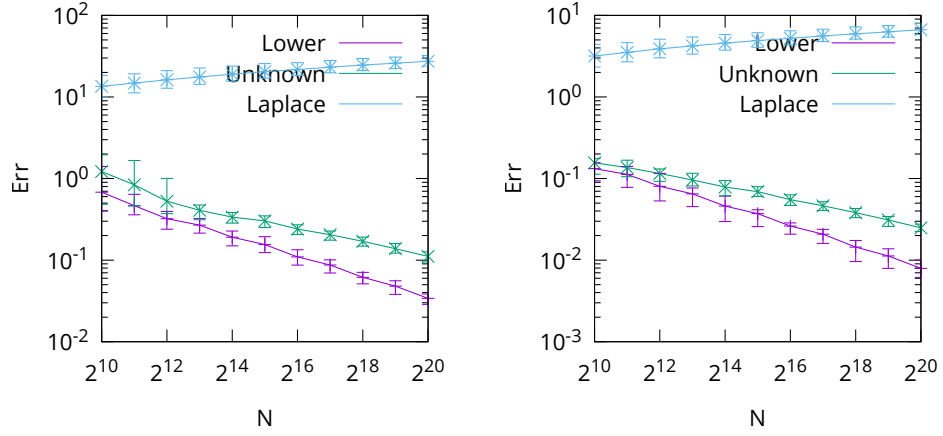

Figure 98: ( $\alpha = 0.9$ ,  $\beta = 1$ ,  $\Delta = 0.6$ , iid) Comparison between our methods and the baseline method with  $\epsilon = 1$  (left) and  $\epsilon = 4$  (right).

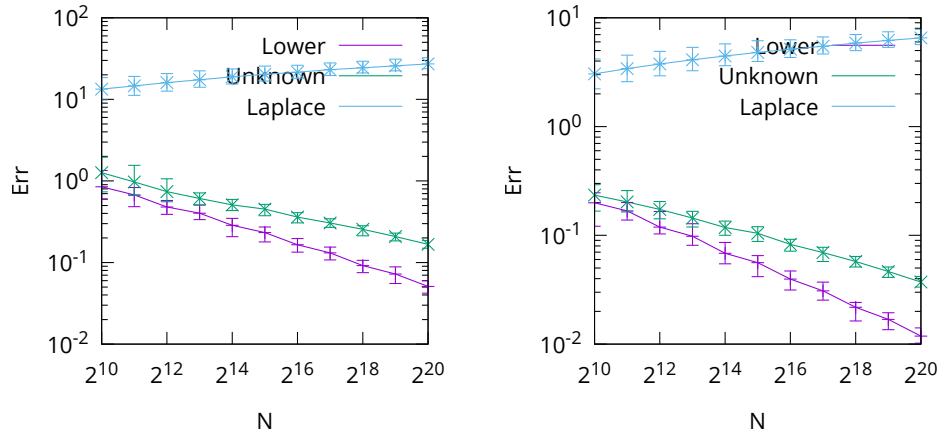

Figure 99: ( $\alpha = 0.9$ ,  $\beta = 1$ ,  $\Delta = 0.9$ , iid) Comparison between our methods and the baseline method with  $\epsilon = 1$  (left) and  $\epsilon = 4$  (right).



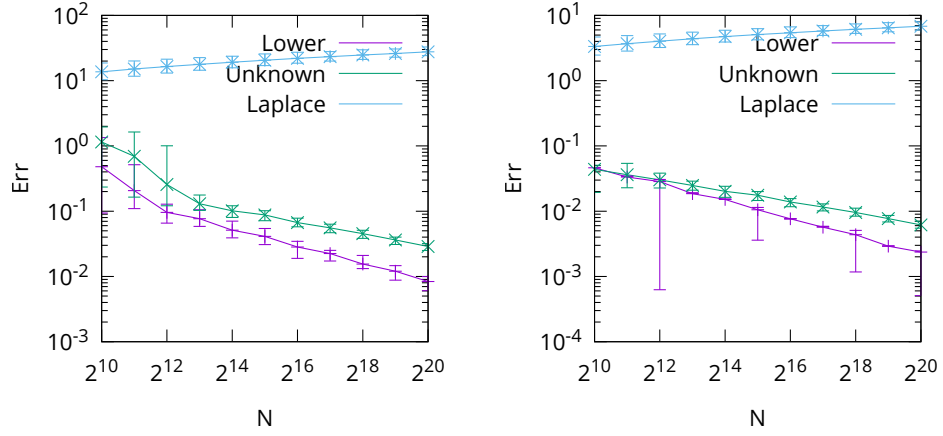

Figure 100: ( $\alpha = 0.9$ ,  $\beta = 2$ ,  $\Delta = 0.3$ , iid) Comparison between our methods and the baseline method with  $\epsilon = 1$  (left) and  $\epsilon = 4$  (right).

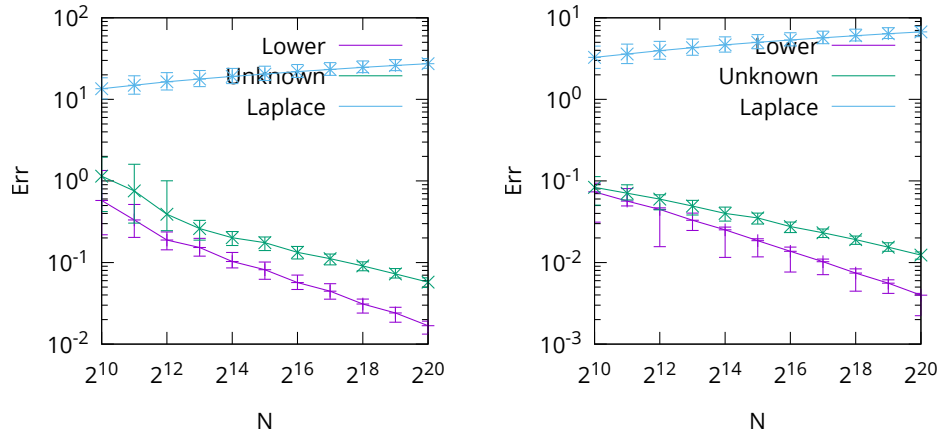

Figure 101: ( $\alpha = 0.9$ ,  $\beta = 2$ ,  $\Delta = 0.6$ , iid) Comparison between our methods and the baseline method with  $\epsilon = 1$  (left) and  $\epsilon = 4$  (right).

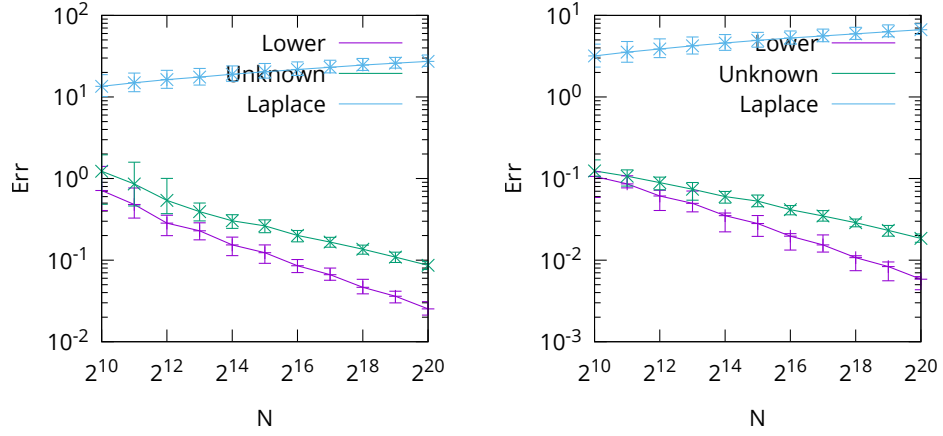

Figure 102: ( $\alpha = 0.9, \beta = 2, \Delta = 0.9$ , iid) Comparison between our methods and the baseline method with  $\epsilon = 1$  (left) and  $\epsilon = 4$  (right).

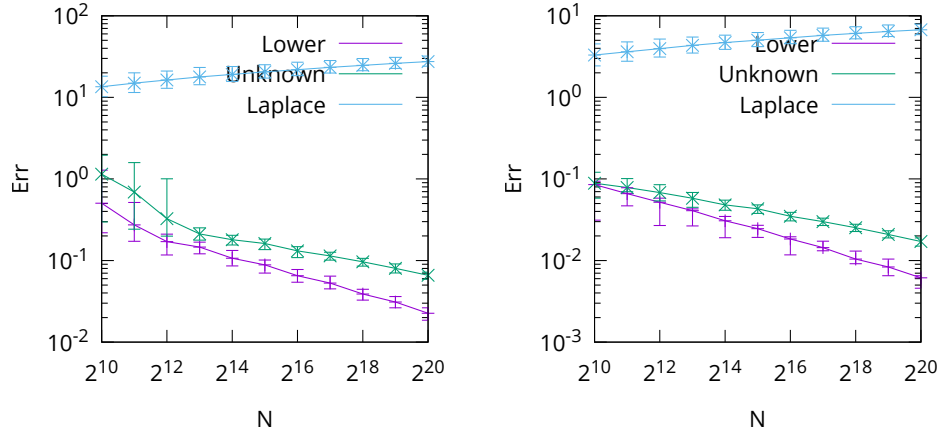

Figure 103: ( $\alpha = 1, \beta = 1, \Delta = 0.3$ , iid) Comparison between our methods and the baseline method with  $\epsilon = 1$  (left) and  $\epsilon = 4$  (right).

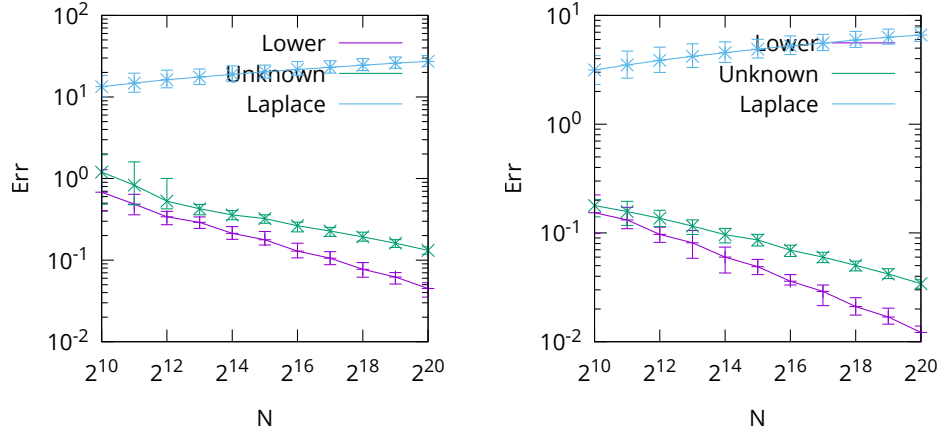

Figure 104: ( $\alpha = 1, \beta = 1, \Delta = 0.6$ , iid) Comparison between our methods and the baseline method with  $\epsilon = 1$  (left) and  $\epsilon = 4$  (right).

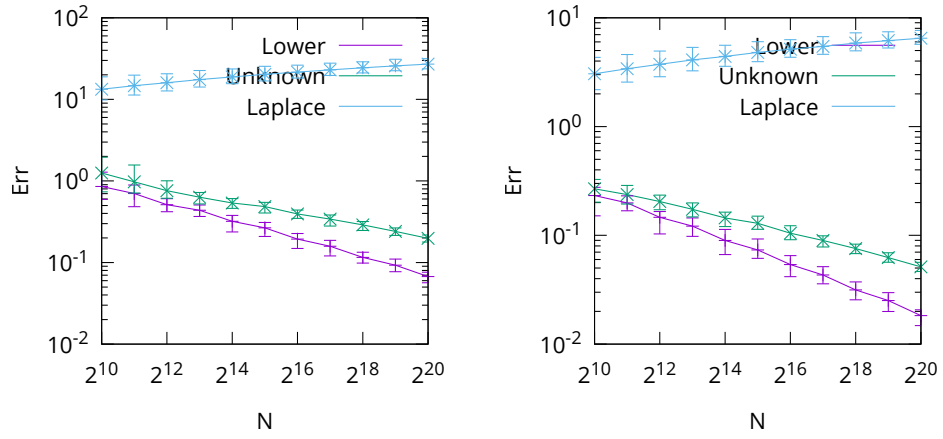

Figure 105: ( $\alpha = 1, \beta = 1, \Delta = 0.9$ , iid) Comparison between our methods and the baseline method with  $\epsilon = 1$  (left) and  $\epsilon = 4$  (right).

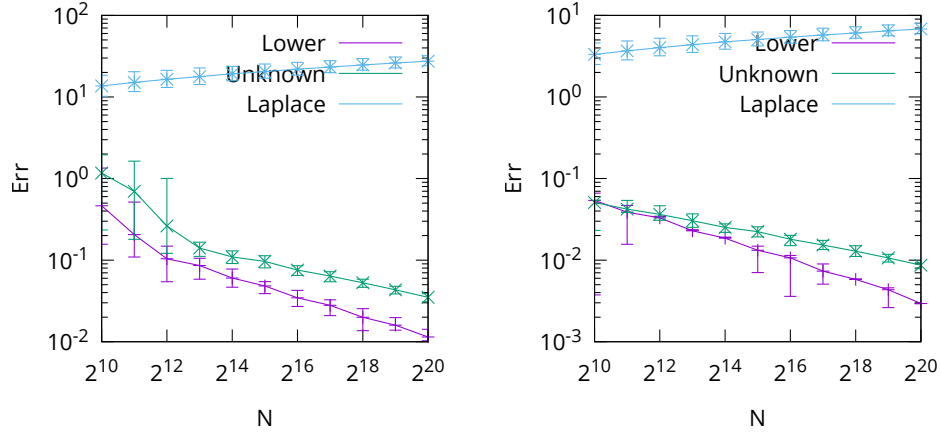

Figure 106: ( $\alpha = 1, \beta = 2, \Delta = 0.3$ , iid) Comparison between our methods and the baseline method with  $\epsilon = 1$  (left) and  $\epsilon = 4$  (right).

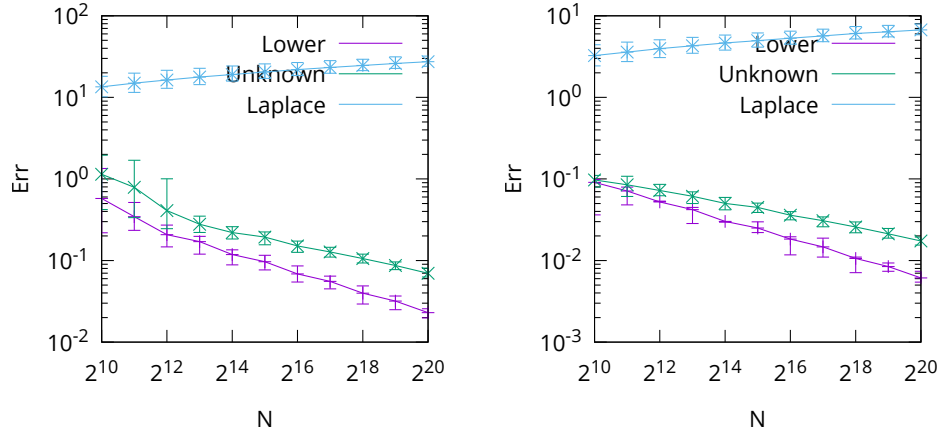

Figure 107: ( $\alpha = 1, \beta = 2, \Delta = 0.6$ , iid) Comparison between our methods and the baseline method with  $\epsilon = 1$  (left) and  $\epsilon = 4$  (right).

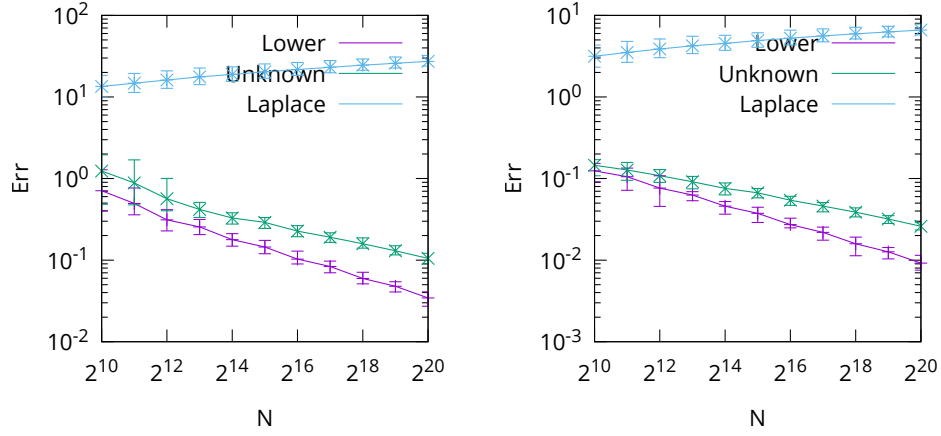

Figure 108: ( $\alpha = 1, \beta = 2, \Delta = 0.9$ , iid) Comparison between our methods and the baseline method with  $\epsilon = 1$  (left) and  $\epsilon = 4$  (right).

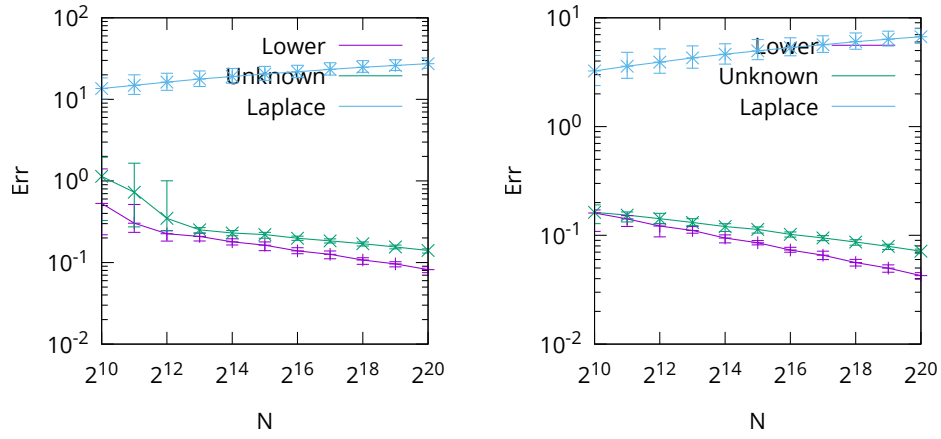

Figure 109: ( $\alpha = 2, \beta = 1, \Delta = 0.3$ , iid) Comparison between our methods and the baseline method with  $\epsilon = 1$  (left) and  $\epsilon = 4$  (right).

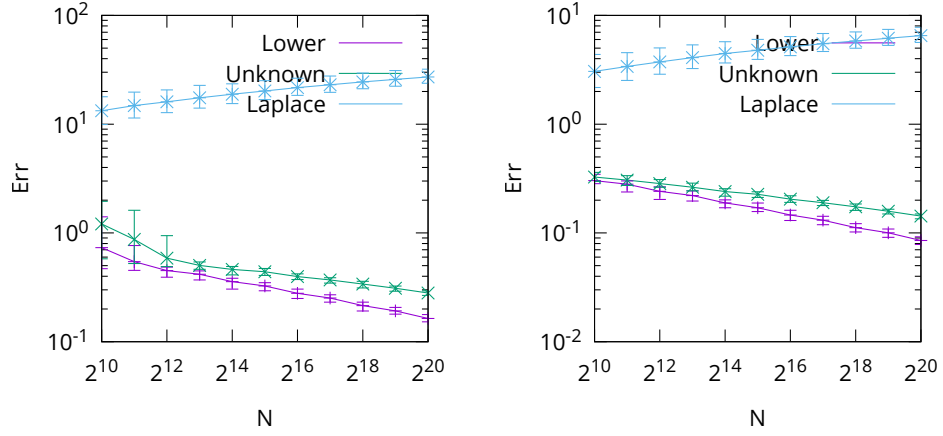

Figure 110: ( $\alpha = 2, \beta = 1, \Delta = 0.6, \text{iid}$ ) Comparison between our methods and the baseline method with  $\epsilon = 1$  (left) and  $\epsilon = 4$  (right).

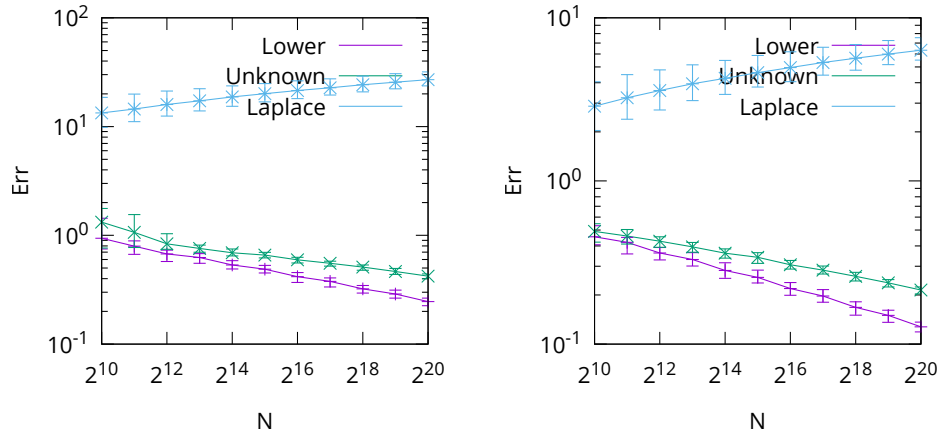

Figure 111: ( $\alpha = 2, \beta = 1, \Delta = 0.9, \text{iid}$ ) Comparison between our methods and the baseline method with  $\epsilon = 1$  (left) and  $\epsilon = 4$  (right).

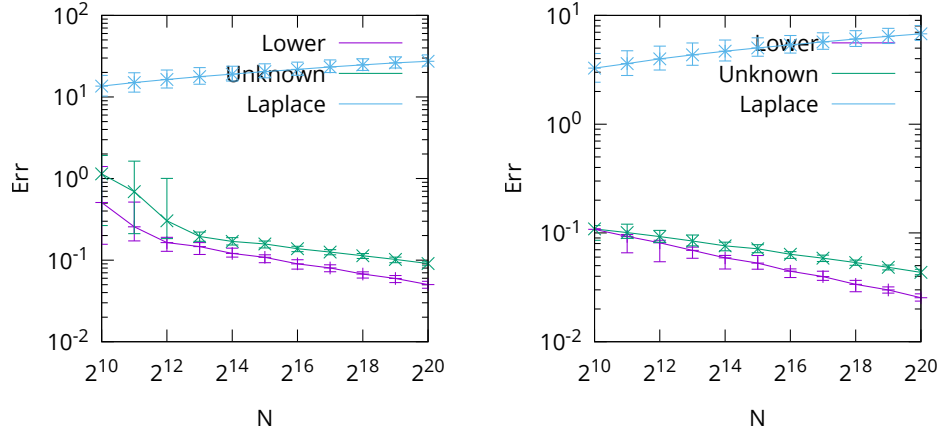

Figure 112: ( $\alpha = 2, \beta = 2, \Delta = 0.3$ , iid) Comparison between our methods and the baseline method with  $\epsilon = 1$  (left) and  $\epsilon = 4$  (right).

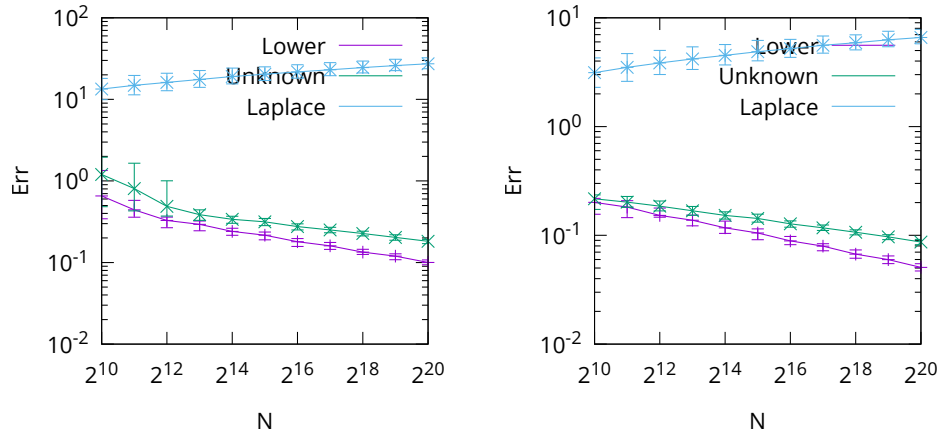

Figure 113: ( $\alpha = 2, \beta = 2, \Delta = 0.6$ , iid) Comparison between our methods and the baseline method with  $\epsilon = 1$  (left) and  $\epsilon = 4$  (right).

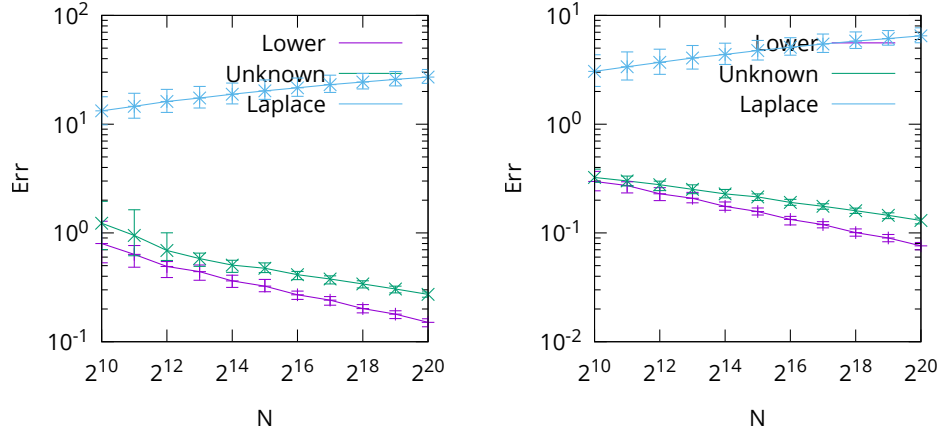

Figure 114: ( $\alpha = 2, \beta = 2, \Delta = 0.9, \text{iid}$ ) Comparison between our methods and the baseline method with  $\epsilon = 1$  (left) and  $\epsilon = 4$  (right).

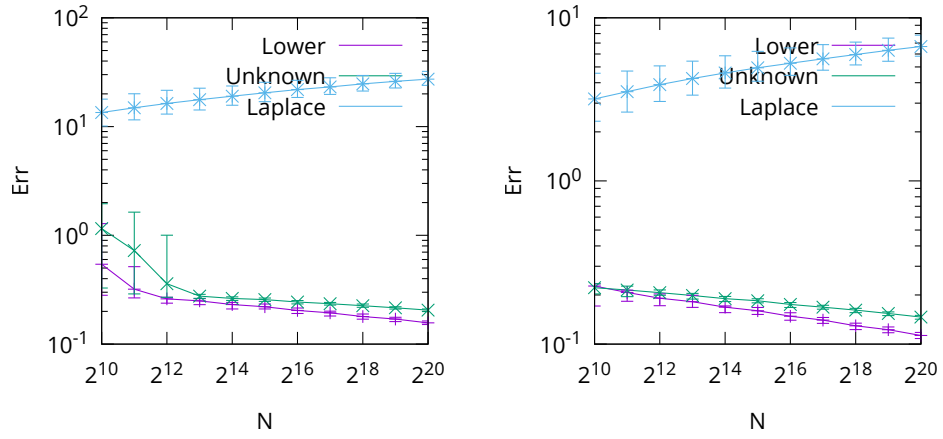

Figure 115: ( $\alpha = 4, \beta = 1, \Delta = 0.3, \text{iid}$ ) Comparison between our methods and the baseline method with  $\epsilon = 1$  (left) and  $\epsilon = 4$  (right).



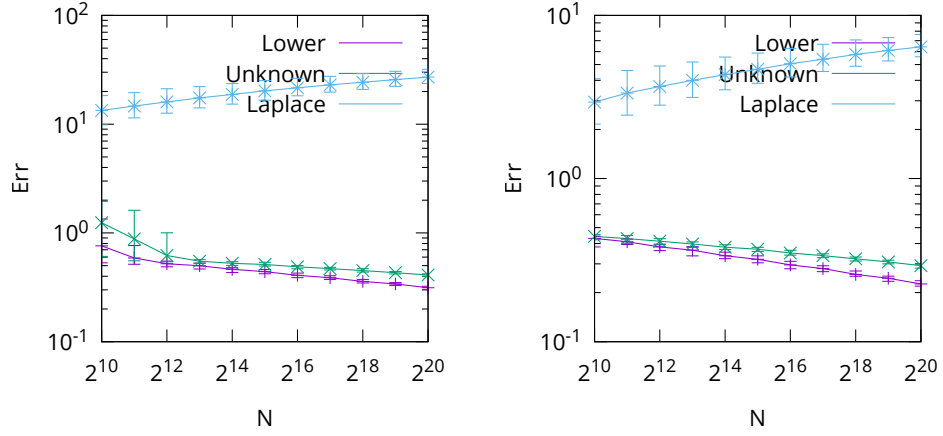

Figure 116: ( $\alpha = 4, \beta = 1, \Delta = 0.6$ , iid) Comparison between our methods and the baseline method with  $\epsilon = 1$  (left) and  $\epsilon = 4$  (right).

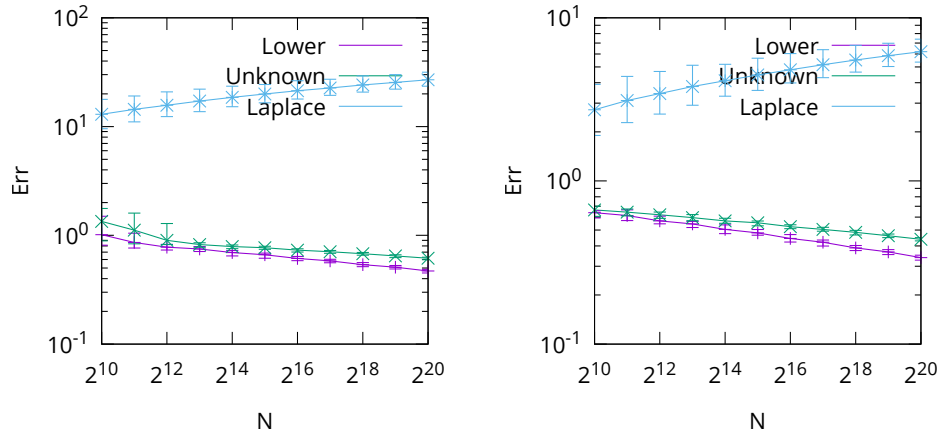

Figure 117: ( $\alpha = 4, \beta = 1, \Delta = 0.9$ , iid) Comparison between our methods and the baseline method with  $\epsilon = 1$  (left) and  $\epsilon = 4$  (right).

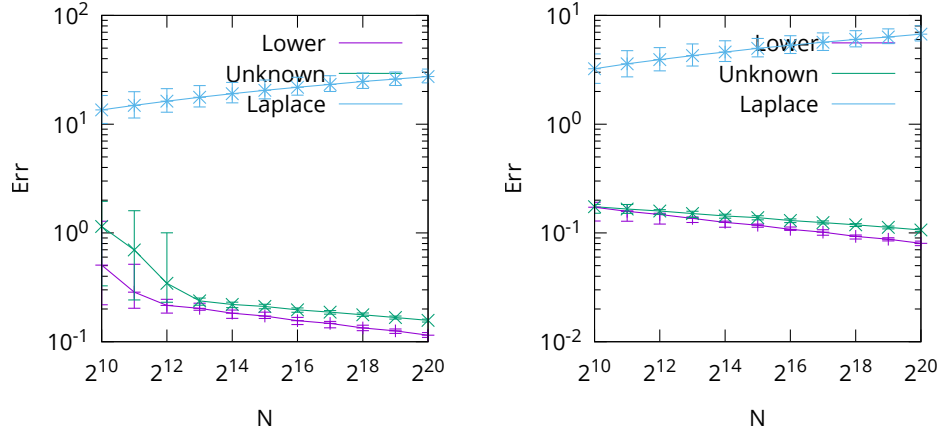

Figure 118: ( $\alpha = 4, \beta = 2, \Delta = 0.3, \text{iid}$ ) Comparison between our methods and the baseline method with  $\epsilon = 1$  (left) and  $\epsilon = 4$  (right).

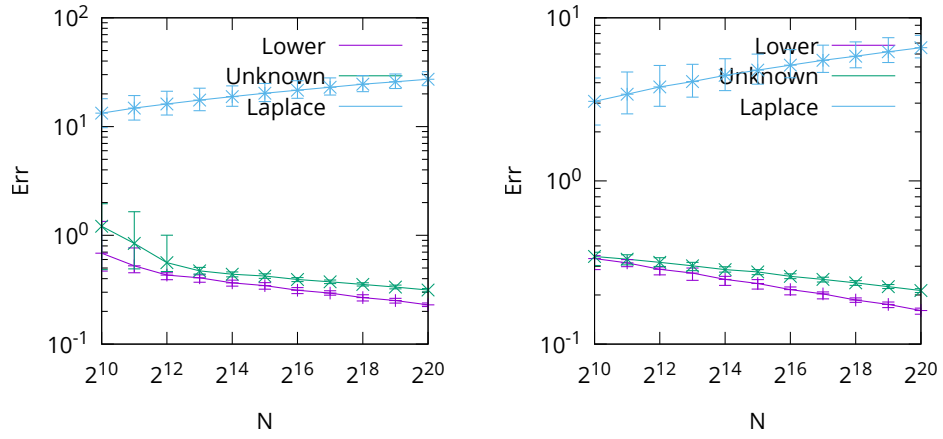

Figure 119: ( $\alpha = 4, \beta = 2, \Delta = 0.6, \text{iid}$ ) Comparison between our methods and the baseline method with  $\epsilon = 1$  (left) and  $\epsilon = 4$  (right).

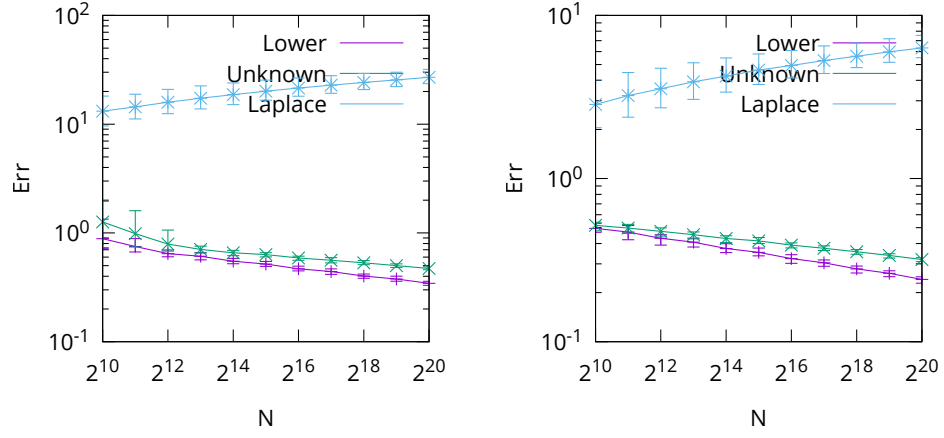

Figure 120: ( $\alpha = 4, \beta = 2, \Delta = 0.9, \text{iid}$ ) Comparison between our methods and the baseline method with  $\epsilon = 1$  (left) and  $\epsilon = 4$  (right).
